# Supplementary material for: Simple Floquet-Wannier-Stark-Andreev viewpoint and emergence of low-energy scales in a voltage-biased three-terminal Josephson junction
Source: arXiv:1611.01932 ancillary file (2017-01-23)
Supplement: Supplementary file 1 [file supplementary.pdf]

# A simple Floquet-Wannier-Stark-Andreev viewpoint and emergence of low-energy scales in a voltage-biased three-terminal Josephson junction: Supplemental Material

Régis Mélin
*Centre National de la Recherche Scientifique, Institut NEEL, F-38042 Grenoble Cedex 9, France and Université Grenoble-Alpes, Institut NEEL, F-38042 Grenoble Cedex 9, France*

Jean-Guy Caputo
*Laboratoire de Mathématiques, INSA de Rouen, Avenue de l'Université, F-76801 Saint-Etienne du Rouvray, France*

Kang Yang
*Laboratoire de Physique Théorique et des Hautes Energies, CNRS UMR 7589, Université Pierre et Marie Curie, Sorbonne Universités, 4 Place Jussieu, 75252 Paris Cedex 05 and Laboratoire de Physique des Solides, CNRS UMR 8502, Univ. Paris-Sud, Université Paris-Saclay F-91405 Orsay Cedex, France*

Benoît Douçot
*Laboratoire de Physique Théorique et des Hautes Energies, CNRS UMR 7589, Université Pierre et Marie Curie, Sorbonne Universités, 4 Place Jussieu, 75252 Paris Cedex 05*

The Supplemental Material presents technical details of the calculations: demonstration of adiabatic theorem (Secs. I and II), a second theorem on the principle of the codes with $\eta_{dot} \neq 0$ (Sec. III), demonstration of the failure of the Keldysh dressing algorithm with discrete spectrum (Sec. IV), details on the Floquet-Lippmann-Schwinger dressing algorithm (Sec. V). The Floquet-Wannier-Stark-Andreev (FWS-Andreev) viewpoint is introduced from a general perspective (Sec. VI). Two complementary determinations of the voltage $V_R$ for the Rabi frequencies are presented in Sec. VII. Finally, the introduction of the generalized Dynes parameter $\eta_{dot}$ is discussed in Sec. VIII.

The goal of the Supplemental Material is to provide technical details on the two methods used in the numerical calculations (Keldysh Green's functions and Floquet-Lippmann-Schwinger calculations). In addition, complementary information will be provided on the Floquet-Wannier-Stark viewpoint, on the calculation of $V_R$ [see Eq. (8) in the paper] and on the nonstandard Dynes parameter $\eta_{dot}$. More precisely, Secs. I and II in Supplemental Material summarize a demonstration of adiabatic theorem. This theorem states that the currents calculated for $\eta_{dot} = 0^+$ are identical to those evaluated for $\eta_{dot} = 0$. New terms are indeed present in the expression of the current if $\eta_{dot} \neq 0$ (and thus also with $\eta_{dot} = 0^+$), which were not there in our previous work[1] with $\eta_{dot} = 0$. This explains why $\eta_{dot} = 0^+$ deserves a special treatment as compared to $\eta_{dot} = 0$. Adiabatic theorem states that the new terms in the current for $\eta_{dot} = 0^+$ (as compared to $\eta_{dot} = 0$) do not contribute in the limit $\eta_{dot} \to 0^+$. Addressing this issue appears to be necessary in view of the exponential dependence on inverse voltage-$V$ of one of the equilibrating mechanism (namely, coupling by multiple Andreev reflections to quasiparticle semi-infinite continua above the gaps). Adiabatic theorem was used to test our code in the limit $\eta_{dot} \to 0$ in which our previous calculations were carried out[1]. The Keldysh Green's function calculations with $\eta_{dot} \neq 0$ involve providing solutions to issues related to current conservation. If nothing special is done, then current conservation is violated because the quantum dot has a continuous spectrum for $\eta_{dot} \neq 0$. The quantum dot can then play the role of a source or a sink of current, as if it were a fourth terminal connected to ground. Those troublesome considerations can be fixed in a mathematically exact manner by a second theorem, which is the subject of Sec. III in Supplemental Material. The status of the Keldysh dressing algorithm is clarified in Sec. IV in Supplemental Material: a demonstration is provided for the failure of the Keldysh dressing algorithm with a discrete spectrum. The spectrum of Floquet-Wannier-Stark-Andreev (FWS-Andreev) resonances is not far from being discrete: the width of those FWS-Andreev resonances is exponentially small in inverse of bias voltage. Sec. V in Supplemental Material provides the technical side of the Floquet-Lippmann-Schwinger calculations. The FWS-Andreev viewpoint is introduced in the main body of the paper in the context of superconducting junctions. Sec. VI in Supplemental Material provides another introduction to FWS ladders, on the basis of general considerations on time-periodic Hamiltonians, not from the superconducting point of view. The Rabi frequencies are determined from Bohr-Sommerfeld quantization in the main body of the paper. Two complementary calculations for the Rabi frequencies are introduced in Sec. VII, on the basis of the rotating wave approximation and the random phase approximation. The introduction of a generalized Dynes parameter $\eta_{dot}$ is motivated in Sec. VIII.

## I. DEMONSTRATION OF ADIABATIC THEOREM

The goal of this section is to introduce a finite $\eta_{dot}$ on the quantum dot, and to demonstrate adiabatic theorem: calculations of DC-transport in the presence of a finite $\eta_{dot} = 0^+$ coincides with those for a vanishingly small $\eta_{dot} = 0$. The demonstration of adiabatic theorem with finite quartet phase $\varphi_Q \neq 0$ is more challenging than for $\varphi_Q = 0$. The demonstration proceeds with first establishing a link with our previous Ref. 2. It is next shown that adiabatic theorem cannot be demonstrated solely from symmetry arguments, except if $\varphi_Q = 0$. On the contrary, the demonstration for $\varphi_Q \neq 0$ requires previous calculation of the fully dressed Green's functions (which is the subject of Sec. II in Supplemental Material.) Introducing a finite line-width broadening for the FWS-Andreev resonances allows to conclude the demonstration of adiabatic theorem.

A contact is first established with the formalism used in our previous work[1], on the basis of Eqs. (31)-(35) in Ref. 2. It is first noticed that Eqs. (33)-(34) in Ref. 2 are not fully general: in this reference, the advanced and retarded Greens function of the quantum dot isolated from the leads is given by

$$g^{A,R}_{x,x}(\omega) = \frac{1}{\omega}, \tag{1}$$

leading to a vanishing small Keldysh Greens function for the quantum dot isolated from the leads:

$$g^{+,-}_{x,x}(\omega) = n(\omega)\left(g^A_{x,x}(\omega) - g^R_{x,x}(\omega)\right) \equiv 0 \tag{2}$$

$$g^K_{x,x}(\omega) = g^{+,-}_{x,x}(\omega) + g^{-,+}_{x,x}(\omega) = (2n(\omega)-1)\left(g^A_{x,x}(\omega) - g^R_{x,x}(\omega)\right) \equiv 0. \tag{3}$$

Eq. (1) differs from the fully general expression for the advanced or retarded Greens function:

$$g^{A,R}_{x,x} = \frac{1}{\omega \mp i\eta_{dot}}, \tag{4}$$

with $\eta_{dot} = 0^+$. Eq. (4) implies the following for the Keldysh Green's function:

$$g^{+,-}_{x,x}(\omega) = n(\omega)\left(\frac{2i\eta_{dot}}{\omega^2 + \eta^2_{dot}}\right) \tag{5}$$

$$g^K_{x,x}(\omega) = (2n(\omega)-1)\left(\frac{2i\eta_{dot}}{\omega^2 + \eta^2_{dot}}\right), \tag{6}$$

where $n(\omega)$ is the Fermi-Dirac distribution. Taking the limit $\eta_{dot} = 0^+$ in Eqs. (5) and (6) leads to

$$g^{+,-}_{x,x}(\omega) = 2i\pi n(\omega)\delta(\omega) \tag{7}$$

$$g^K_{x,x}(\omega) = 2i\pi\left(2n(\omega)-1\right)\delta(\omega). \tag{8}$$

Comparing Eqs. (2) and (3) to Eqs. (7) and (8), it is concluded that a $\delta$-function was not present in the quantum dot Keldysh Greens function in Ref. 1. The adiabatic theorem demonstrated below states that the current is independent on whether Eqs. (2), (3) or Eqs. (7), (8) are used: the calculations presented in our previous paper[1] are valid. However, physically relevant information is encoded in the speed of convergence towards adiabatic solution as $\eta_{dot} \to 0^+$, which is exponentially small in $\Delta/V$. This opens the way to experimental relevance of a regime (corresponding to $\eta_{dot} \gg \eta^*_{dot}$ in Fig. 5 of the paper) in which the quantum dot degrees of freedom are not equilibrated with the quasiparticle continua above the gaps. It is this regime (not captured by our previous Ref. 1) which is of importance if one wants to discuss experiments. It is not claimed here that the recent experiment of the Weizmann group[3] operates in the regime $\eta_{dot} \gg \eta^*_{dot}$. It is just mentioned that it will interesting to consider in thee future the question of experimental relevance of this nonstandard regime, in connection with the available experimental data of the Weizmann group[3].

Coming back to the demonstration of adiabatic theorem, the Dyson equation takes the form

$$\hat{G}_{x,x} = \hat{g}_{x,x} + \hat{g}_{x,x}\hat{\Gamma}\hat{G}_{x,x}, \tag{9}$$

with $\hat{\Gamma} = \hat{\Sigma}_{x,k}\hat{g}_{k,k}\hat{\Sigma}_{k,x}$, where a summation over $k \in \{S_a, S_b, S_c\}$ is carried out. Eq. (9) is equivalent to

$$\hat{G}_{x,x} = \left[(\hat{g}_{x,x})^{-1} - \hat{\Gamma}\right]^{-1}, \tag{10}$$

which is Eq. (31) in Ref. 2.

The Dyson-Keldysh equation

$$\hat{G}^{+,-} = \left(\hat{I} + \hat{G}^R\hat{\Sigma}\right)\hat{g}^{+,-}\left(\hat{I} + \hat{\Sigma}\hat{G}^A\right) \tag{11}$$

leads to

$$\hat{G}^{+,-}_{x,x} = (\hat{\text{A}}) + (\hat{\text{B}}), \tag{12}$$

with

$$(\hat{\text{A}}) = \hat{g}^{+,-}_{x,x} + \hat{G}^R_{x,x}\hat{\Sigma}_{x,k}\hat{\Gamma}^{+,-}\hat{G}^A_{x,x} \tag{13}$$

$$(\hat{\text{B}}) = \hat{G}^R_{x,x}\hat{\Gamma}^R\hat{g}^{+,-}_{x,x} + \hat{g}^{+,-}_{x,x}\hat{\Gamma}^A\hat{G}^A_{x,x} + \hat{G}^R_{x,x}\hat{\Gamma}^R\hat{g}^{+,-}_{x,x}\hat{\Gamma}^A\hat{G}^A_{x,x}, \tag{14}$$

with $\hat{\Gamma}^{A,R} = \hat{\Sigma}_{x,k}\hat{g}^{A,R}_{k,k}\hat{\Sigma}_{k,x}$ and $\hat{\Gamma}^{+,-} = \hat{\Sigma}_{x,k}\hat{g}^{+,-}_{k,k}\hat{\Sigma}_{k,x}$ (with implicit summation over $k$). Eq. (13) is equivalent to Eq. (32) in Ref. 2. Eq. (14) corresponds to new terms which are absent if $\eta_{dot} = 0$.

The spectral current from the dot $x$ to the lead $S_l$ takes the form

$$\hat{I}_l = \hat{\tau}_3\left[\hat{\Sigma}_{l,x}\hat{G}^{+,-}_{x,l} - \hat{\Sigma}_{x,l}\hat{G}^{+,-}_{l,x}\right]. \tag{15}$$

A straightforward calculation leads to

$$\hat{I}_l = \hat{\tau}_3\left[\hat{\Sigma}_{l,x}\hat{G}^R_{x,x}\hat{\Sigma}_{x,l}\hat{g}^{+,-}_{l,l} - \hat{\Sigma}_{x,l}\hat{g}^{+,-}_{l,l}\hat{\Sigma}_{l,x}\hat{G}^A_{x,x} + \hat{\tau}_3\hat{\Sigma}_{l,x}\hat{G}^{+,-}_{x,x}\hat{\Sigma}_{x,l}\hat{g}^A_{l,l} - \hat{\Sigma}_{x,l}\hat{g}^R_{l,l}\hat{\Sigma}_{l,x}\hat{G}^{+,-}_{x,x}\right]. \tag{16}$$

Further calculations show that Eq. (16) is equivalent to Eq. (35) in Ref. 2.

If $\eta_{dot} = 0$ (see Refs. 1 and 2), then $(\hat{\text{B}}) = 0$ and $(\hat{\text{A}}) = \hat{G}^R_{x,x}\hat{\Sigma}_{x,k}\hat{\Gamma}^{+,-}\hat{G}^A_{x,x}$ in Eq. (14). Current is then automatically conserved and the demonstration of the adiabatic theorem is already finished for $\eta_{dot} = 0$. On the contrary, if $\eta_{dot} \neq 0$, then current may depend on the bare populations $n(\omega)$ of the quantum dot at time $t = -\infty$ in the adiabatic procedure. Our algorithm for finite $\eta_{dot}$ evaluates those populations self-consistently (see the forthcoming Sec. III in Supplemental Material).

In the presence of particle-hole symmetry, the quartet or multipair current is odd in phase and even in voltage, and the phase-MAR current is even in phase and odd in voltage. Those statements put constraints on current conservation. The state of the quantum dot at the beginning of adiabatic continuation has to be specified; to start with: $n(\omega) = \theta(-\omega)$. The contacts between the dot and leads $S_a$ and $S_a$ are supposed to have identical transparency. Exchanging leads $S_a$ and $S_b$ implies that $I_a + I_b + I_c$ is even in voltage, and thus odd in phase:

$$(I_a + I_b + I_c)(V, \varphi_Q) = -(I_a + I_b + I_c)(V, -\varphi_Q). \tag{17}$$

Current conservation is automatically fulfilled if $\varphi_Q = 0$, because Eq. (17) with $\varphi_Q = 0$ implies $I_a + I_b + I_c = 0$, whatever the state of the quantum dot at time $t = -\infty$ in adiabatic continuation. This demonstrates the adiabatic theorem if $\varphi_Q = 0$. Eq. (17) implies that $I_a + I_b + I_c = 0$ in the adiabatic limit is not given for free if $\varphi_Q \neq 0$.

Further remarks are presented now on a situation in which all superconductors are in the normal state. The fully dressed Green's function is given by $G_{x,x} = [(g_{x,x})^{-1} - \Gamma]^{-1}$ [see Eq. (10)]. Normal leads imply $g^{-1}_{x,x} = \omega$ and $G_{x,x} \to -\Gamma^{-1}$ if $\omega \to 0^+$. Then, the factors $(\Gamma^{A/R})^{-1}$ cancel with $\Gamma^{A/R}$ in the transport formula [see Eqs. (12)-(14) and Eq. (16)]. The terms in $g^{+,-}_{x,x}$ cancel in $I_a + I_b + I_c$, leading to $I_a + I_b + I_c = 0$, whatever the initial state of the dot. With voltage-biased superconducting electrodes, then $G_{x,x}$ does not go to $-\Gamma^{-1}$ as $\omega \to 0^+$. The "discrete" contribution to $I_a + I_b + I_c$ is not constraint to be vanishingly small by this argument. It is confirmed that $I_a + I_b + I_c = 0$ in the adiabatic limit is not given for free if $\varphi_Q \neq 0$.

A direct evaluation of $I_a + I_b + I_c$ is carried out now. The starting point is Eq. (28) for $I_a + I_b + I_c$ demonstrated in the forthcoming Sec. II in Supplemental Material.

Andreev resonances of width $\gamma_0$ appear at energies $\{\omega^{(0)}_\alpha\}$ in the advanced and retarded Green's functions:

$$\hat{G}^R_{x,x} = \sum_\alpha \frac{\hat{K}^R_\alpha}{\omega - \omega^{(0)}_\alpha + i\gamma_0} + ... \text{ , and } \hat{G}^A_{x,x} = \sum_\beta \frac{\hat{K}^A_\beta}{\omega - \omega^{(0)}_\beta - i\gamma_0} + ... \tag{18}$$

Then, Eq. (28) takes the form

$$I_{tot}[n_{x,x}] = -2i\eta_{dot} \int d\omega \sum_{k,\tau,\alpha,\beta} \langle \tau,0|\hat{\tau}_3 \hat{\Sigma}_{a_k,x} \frac{\hat{K}_\alpha^R}{\omega - \omega_\alpha^{(0)} + i\gamma_0} \hat{n}_{x,x} \frac{\hat{K}_\beta^A}{\omega - \omega_\beta^{(0)} - i\gamma_0} \hat{\Sigma}_{x,a_k} \hat{g}^A_{a_k,a_k} |\tau,0\rangle$$

$$+ \; 2i\eta_{dot} \int d\omega \sum_{k,\tau,\alpha,\beta} \langle \tau,0|\hat{\tau}_3 \hat{\Sigma}_{x,a_k} \hat{g}^R_{a_k,a_k} \hat{\Sigma}_{a_k,x} \frac{\hat{K}_\alpha^R}{\omega - \omega_\alpha^{(0)} + i\gamma_0} \hat{n}_{x,x} \frac{\hat{K}_\beta^A}{\omega - \omega_\beta^{(0)} - i\gamma_0} |\tau,0\rangle, \tag{19}$$

where $|\tau,0\rangle$ corresponds to Nambu label $\tau$ and Floquet label 0. The leading order term in Eq. (19) corresponds to $\alpha = \beta$:

$$I_{tot}[n_{x,x}] \simeq -2i\eta_{dot} \int d\omega \sum_\alpha \frac{1}{(\omega - \omega_\alpha^{(0)})^2 + (\gamma_0)^2} \tag{20}$$

$$\times \sum_{k,\tau} \left[ \langle \tau,0|\hat{\tau}_3 \hat{\Sigma}_{a_k,x} \hat{K}^R_\alpha \hat{n}_{x,x} \hat{K}^A_\alpha \hat{\Sigma}_{x,a_k} \hat{g}^A_{a_k,a_k} |\tau,0\rangle - \langle \tau,0|\hat{\tau}_3 \hat{\Sigma}_{x,a_k} \hat{g}^R_{a_k,a_k} \hat{\Sigma}_{a_k,x} \hat{K}^R_\alpha \hat{n}_{x,x} \hat{K}^A_\alpha |\tau,0\rangle \right].$$

Thus, $I_{tot}[n_{x,x}]$ is of order $I_{tot}[n_{x,x}] \sim (e/h)\Gamma\eta_{dot}/\gamma_0$, with $\Gamma = t^2/W$ the line-width broadening due to the coupling to the leads, where $t = |\Sigma_{a,\alpha}| = |\Sigma_{b,\beta}|$ for simplicity.

The terms proportional to $g^{+,-}_{x,x}$ do not contribute to $I_a$, $I_b$ or $I_c$ if the limit $\eta_{dot} \to 0^+$ is taken first. This concludes the demonstration of the adiabatic theorem with quartet phase $\varphi_Q \neq 0$.

## II. DETAILS ON THE DIFFERENT COMPONENTS OF THE CURRENT

The transport formula are evaluated in this section for a three-terminal Josephson junction with finite Dynes parameter $\eta_{dot} \neq 0$ on the quantum dot. The calculation proceeds with manipulations of the Dyson equation. The currents are linear in the bare populations of the superconducting leads, and those of the quantum dot. The introduction of the latter is a consequence of handling calculations with $\eta_{dot} \neq 0$.

It is also noted that Dyson equation equations are formally divergent series, because the quantum dot advanced and retarded Green's functions diverge in the limits $\omega \to 0$ and $\eta_{dot} \to 0$ (see Eq. (4)). In this respect, the parameter $\eta_{dot}$ is there to regularize those divergences. The validity of the following calculations relies on observation that all of the calculated components of the current are finite in the end.

### A. Decomposition of the current

The Dyson equation for the Keldysh Green's function and the current[4–6] is decomposed as the sum of a quasiequilibrium component involving only advanced Green's functions, and a nonequilibrium component involving products of advanced and retarded Green's functions. The total Keldysh Green's function at times $t_1$ and $t_2$ takes the following form: $\hat{G}^{+,-}(t_1,t_2) = \hat{G}^{+,-}_{Quasieq.}(t_1,t_2) + \hat{G}^{+,-}_{Noneq.}(t_1,t_2)$, with

$$\hat{G}^{+,-}_{Quasieq.} = \hat{n} \otimes \hat{G}^A - \hat{G}^R \otimes \hat{n} \tag{21}$$

$$\hat{G}^{+,-}_{Noneq.} = \hat{G}^R \otimes \left( \hat{\Sigma} \otimes \hat{n} - \hat{n} \otimes \hat{\Sigma} \right) \otimes \hat{G}^A. \tag{22}$$

The symbol $\otimes$ in those equations is a convolution over the time variables. After Fourier transform from time to frequency, Eqs. (21) and (22) take the form of simple matrix products. Those matrices have components in Nambu for electrons and holes; other labels ($x$, $a$, $b$ and $c$) correspond to the "graph" defining the contacts (see Fig. 1 of the paper). Other labels correspond to the harmonics $n\omega_0/2$ of the Josephson frequency, with $n$ an integer and $\omega_0 = 2eV/\hbar$. The symbol $\hat{n}$ (with a "hat") in Eqs. (21) and (22) stands for the quantum dot populations. The matrices $\hat{n}$ are local in space and diagonal in Nambu: $n^{1,1}_{l,l}(\omega) = n_F(\omega - \mu_l)$ and $n^{2,2}_{l,l}(\omega) = n_F(\omega + \mu_l)$. It is considered that $\mu_l = 0$ for the superconducting leads ($l \in \{a,b,c\}$), and that $\mu_l = \mu_{dot}$ for the quantum dot, where $\mu_{dot}$ is a central quantity in the paper.

### B. Expression for the different components of the current

The populations of the superconducting leads $S_a$, $S_b$ and $S_c$, and those of the dot $x$ are denoted by $n_{a,a}(\omega)$, $n_{b,b}(\omega)$, $n_{c,c}(\omega)$ and by $n_{x,x}(\omega)$ respectively. The current through the link $a_k - x$ ($a_k \in \{a,b,c\}$) takes the form

$I_{a_k} = I_{a_k,x} - I_{x,a_k}$, with

$$I_{a_k,x} = \frac{e}{h}\sum_\tau \langle \tau,0|\hat{\Sigma}_{a_k,x}\hat{G}^{+,-}_{x,a_k} - \hat{\Sigma}_{x,a_k}\hat{G}^{+,-}_{a_k,x}|\tau,0\rangle \quad (23)$$

$$I_{x,a_k} = \frac{e}{h}\sum_\tau \langle \tau,0|\hat{\Sigma}_{x,a_k}\hat{G}^{+,-}_{a_k,x} - \hat{\Sigma}_{a_k,x}\hat{G}^{+,-}_{x,a_k}|\tau,0\rangle, \quad (24)$$

where $|\tau,n\rangle$ is a vector having components in Nambu and the set of harmonics $n\hbar\omega_0/2$ of the Josephson frequency. Due to the form of the Dyson-Keldysh equation, the current $I_{a_k}$ is given by the following combination:

$$I_{a_k} = I_{a_k}[n_{x,x}] + I_{a_k}[n_{a,a}] + I_{a_k}[n_{b,b}] + I_{a_k}[n_{c,c}], \quad (25)$$

where $I_{a_k}[n_{l,l}]$ depends only on the populations $n_{l,l}(\omega)$ in lead $l \in \{a,b,c,x\}$. It is however not given for free that the combination

$$I_{tot}[n_{x,x}] = I_a[n_{x,x}] + I_b[n_{x,x}] + I_c[n_{x,x}] \quad (26)$$

is vanishingly small. The main conclusion of Sec.II C is that Eq. (26) is equivalent to

$$I_{tot}[n_{x,x}] = \int d\omega \sum_{k,\tau} \langle \tau,0|\hat{\tau}_3\hat{\Sigma}_{a_k,x}\hat{G}^R_{x,x}\hat{n}_{x,x}\left[\left(\hat{g}^A\right)^{-1} - \left(\hat{g}^R\right)^{-1}\right]_{x,x}\hat{G}^A_{x,a_k}|\tau,0\rangle - \int d\omega \sum_{k,\tau} \langle \tau,0|\hat{\tau}_3\hat{\Sigma}_{x,a_k}\hat{G}^R_{a_k,x}\hat{n}_{x,x}\left[\left(\hat{g}^A\right)^{-1} - \left(\hat{g}^R\right)^{-1}\right]_{x,x}\hat{G}^A_{x,x}|\tau,0\rangle. \quad (27)$$

Using $\hat{g}^{A,R} = \left[\omega - \hat{\mathcal{H}} - i\eta_{dot}\right]^{-1}$, with $\hat{\mathcal{H}}$ the Hamiltonian, leads to

$$I_{tot}[n_{x,x}] = -2i\eta_{dot}\int d\omega \sum_{k,\tau}\langle \tau,0|\hat{\tau}_3\hat{\Sigma}_{a_k,x}\hat{G}^R_{x,x}\hat{n}_{x,x}\hat{G}^A_{x,a_k}|\tau,0\rangle + 2i\eta_{dot}\int d\omega \sum_{k,\tau}\langle \tau,0|\hat{\tau}_3\hat{\Sigma}_{x,a_k}\hat{G}^R_{a_k,x}\hat{n}_{x,x}\hat{G}^A_{x,x}|\tau,0\rangle. \quad (28)$$

For the considered particle-hole symmetric quantum dot, the trace over Nambu in Eq. (28) implies antisymetrization of $I_{tot}[n_{x,x}]$ with respect to the quartet phase variable $\varphi_b$. As a consequence, $I_{tot}[n_{x,x}] = 0$ if $\varphi_b$ takes the special values $\varphi_b = 0$ or $\varphi_b = \pi$, but, in general, $I_{tot}[n_{x,x}] \neq 0$. In what follows, the necessary self-consistent procedure is provided, by which current conservation is restored.

### C. Expression for the current

Eq. (22) takes the form

$$\Sigma_{a,x}\hat{G}^{+,-}_{Noneq.,x,a} = \sum_{\alpha=1}^{6} A^a_\alpha, \quad (29)$$

with

$$A^a_1 = \hat{\Sigma}_{a,x}\hat{G}^R_{x,x}\left[\hat{\Sigma}_{x,a}\hat{n}_{a,a} - \hat{n}_{x,x}\hat{\Sigma}_{x,a}\right]\hat{G}^A_{a,a} \quad (30)$$

$$A^a_2 = \hat{\Sigma}_{a,x}\hat{G}^R_{x,x}\left[\hat{\Sigma}_{x,b}\hat{n}_{b,b} - \hat{n}_{x,x}\hat{\Sigma}_{x,b}\right]\hat{G}^A_{b,a} \quad (31)$$

$$A^a_3 = \hat{\Sigma}_{a,x}\hat{G}^R_{x,x}\left[\hat{\Sigma}_{x,c}\hat{n}_{c,c} - \hat{n}_{x,x}\hat{\Sigma}_{x,c}\right]\hat{G}^A_{c,a} \quad (32)$$

$$A^a_4 = \hat{\Sigma}_{a,x}\hat{G}^R_{x,a}\left[\hat{\Sigma}_{a,x}\hat{n}_{x,x} - \hat{n}_{a,a}\hat{\Sigma}_{a,x}\right]\hat{G}^A_{x,a} \quad (33)$$

$$A^a_5 = \hat{\Sigma}_{a,x}\hat{G}^R_{x,b}\left[\hat{\Sigma}_{b,x}\hat{n}_{x,x} - \hat{n}_{b,b}\hat{\Sigma}_{b,x}\right]\hat{G}^A_{x,a} \quad (34)$$

$$A^a_6 = \hat{\Sigma}_{a,x}\hat{G}^R_{x,c}\left[\hat{\Sigma}_{c,x}\hat{n}_{x,x} - \hat{n}_{c,c}\hat{\Sigma}_{c,x}\right]\hat{G}^A_{x,a}. \quad (35)$$

Each of the six terms in Eqs. (30)-(35) is decomposed into the sum of a term involving the populations of the superconductors (denoted generically as $n_S \in \{n_{a,a}, n_{b,b}, n_{c,c}\}$), and another term with the populations $n_x$ of the quantum dot: $A_\alpha^a = A_\alpha^a[n_S] + A_\alpha^a[n_{x,x}]$, with for instance $A_1^a[n_S] = \hat{\Sigma}_{a,x}\hat{G}^R_{x,x}\hat{\Sigma}_{x,a}\hat{n}_{a,a}\hat{G}^A_{a,a}$ and $A_1^a[n_{x,x}] = -\hat{\Sigma}_{a,x}\hat{G}^R_{x,x}\hat{n}_{x,x}\hat{\Sigma}_{x,a}\hat{G}^A_{a,a}$. The quantities $A_\alpha^a$ (with $\alpha = 1, ..., 3$) are expanded as follows:

$$A_1^a[n_{x,x}] = -\hat{\Sigma}_{a,x}\hat{G}^R_{x,x}\hat{n}_{x,x}\left(\hat{g}^A_{x,x}\right)^{-1}\left[\hat{g}^A_{x,x}\hat{\Sigma}_{x,a}\hat{G}^A_{a,a}\right] \quad (36)$$

$$A_2^a[n_{x,x}] = -\hat{\Sigma}_{a,x}\hat{G}^R_{x,x}\hat{n}_{x,x}\left(\hat{g}^A_{x,x}\right)^{-1}\left[\hat{g}^A_{x,x}\hat{\Sigma}_{x,b}\hat{G}^A_{b,a}\right] \quad (37)$$

$$A_3^a[n_{x,x}] = -\hat{\Sigma}_{a,x}\hat{G}^R_{x,x}\hat{n}_{x,x}\left(\hat{g}^A_{x,x}\right)^{-1}\left[\hat{g}^A_{x,x}\hat{\Sigma}_{x,c}\hat{G}^A_{c,a}\right]. \quad (38)$$

Using $\hat{g}^A_{x,x}\hat{\Sigma}_{x,a}\hat{G}^A_{a,a} + \hat{g}^A_{x,x}\hat{\Sigma}_{x,b}\hat{G}^A_{b,a} + \hat{g}^A_{x,x}\hat{\Sigma}_{x,c}\hat{G}^A_{c,a} = \hat{G}^A_{x,a}$ leads to

$$\left(A_1^a + A_2^a + A_3^a\right)[\hat{n}_{x,x}] = -\hat{\Sigma}_{a,x}\hat{G}^R_{x,x}\hat{n}_{x,x}\left(\hat{g}^A_{x,x}\right)^{-1}\hat{G}^A_{x,a}. \quad (39)$$

Using now $\hat{G}^R_{x,x} = \hat{g}^R_{x,x} + \hat{G}^R_{x,a}\hat{\Sigma}_{a,x}\hat{g}^R_{x,x} + \hat{G}^R_{x,b}\hat{\Sigma}_{b,x}\hat{g}^R_{x,x} + \hat{G}^R_{x,c}\hat{\Sigma}_{c,x}\hat{g}^R_{x,x}$, and combining with Eqs. (33)-(35) leads to

$$\left(A_1^a + ... + A_6^a\right)[\hat{n}_{x,x}] = -\hat{\Sigma}_{a,x}\hat{n}_{x,x}\left(\hat{g}^R_{x,x}/\hat{g}^A_{x,x}\right)\hat{G}^A_{x,a} - \hat{\Sigma}_{a,x}\left[\hat{G}^R_{x,x} - \hat{g}^R_{x,x}\right]\hat{n}_{x,x}\left[\left(\hat{g}^A_{x,x}\right)^{-1} - \left(\hat{g}^R_{x,x}\right)^{-1}\right]\hat{G}^A_{x,a}. \quad (40)$$

Combining with $\hat{\Sigma}_{a,x}\hat{G}^{+,-}_{Quasieq.,x,a}[n_{x,x}] = \hat{\Sigma}_{a,x}\hat{n}_{x,x}\hat{G}^A_{x,a}$ leads to the following component to the current:

$$I_{a,x}[n_{x,x}] \equiv \mathrm{Tr}\left\{\hat{\tau}_3\hat{\Sigma}_{a,x}\hat{G}^{+,-}_{x,a}\right\}[n_{x,x}] = \mathrm{Tr}\left\{\hat{\tau}_3\hat{\Sigma}_{a,x}\hat{G}^R_{x,x}\hat{n}_{x,x}\left[\left(\hat{g}^A_{x,x}\right)^{-1} - \left(\hat{g}^R_{x,x}\right)^{-1}\right]\hat{G}^A_{x,a}\right\}. \quad (41)$$

Similar expressions are obtained for $I_{b,x}[n_{x,x}]$ and $I_{c,x}[n_{x,x}]$.

Similar calculations were carried out for

$$I_{x,a}[n_{x,x}] \equiv -\mathrm{Tr}\left\{\hat{\tau}_3\hat{\Sigma}_{x,a}\hat{G}^{+,-}_{a,x}\right\}[n_{x,x}] = \mathrm{Tr}\left\{\hat{\tau}_3\hat{\Sigma}_{x,a}\hat{G}^R_{a,x}\hat{n}_{x,x}\left[\left(\hat{g}^A_{x,x}\right)^{-1} - \left(\hat{g}^R_{x,x}\right)^{-1}\right]\hat{G}^A_{x,x}\right\}, \quad (42)$$

and similar expressions were obtained for $I_{x,b}[n_{x,x}]$ and $I_{x,c}[n_{x,x}]$, as well as for $I_{x,a}[n_S]$, $I_{x,b}[n_S]$ and $I_{x,c}[n_S]$.

### D. A consequence of Eq. (27)

Let us consider (only in this subsection) a double quantum dot with two levels at energy $\pm\epsilon_0$. Then:

$$g^A_{x,x}(\omega, \eta_{dot}) = \frac{1}{\omega - \epsilon_0 - i\eta_{dot}} + \frac{1}{\omega + \epsilon_0 - i\eta_{dot}}, \quad (43)$$

and

$$\left[g^A_{x,x}(\omega, \eta_{dot})\right]^{-1} = \frac{1}{\frac{1}{\omega - \epsilon_0 - i\eta_{dot}} + \frac{1}{\omega + \epsilon_0 - i\eta_{dot}}} = \frac{(\omega - i\eta_{dot})^2 - (\epsilon_0)^2}{2(\omega - i\eta_{dot})} \quad (44)$$

has a pole at $\omega = 0$. Then:

$$\left[g^A_{x,x}(\omega, \eta_{dot})\right]^{-1} - \left[g^R_{x,x}(\omega, \eta_{dot})\right]^{-1} \simeq \left(\omega^2 - (\epsilon_0)^2\right)\frac{\eta_{dot}}{\omega^2 + \eta^2_{dot}} \quad (45)$$

is proportional to $\delta(\omega)$ in the limit $\eta_{dot} \to 0^+$. On the contrary, the following is obtained if $\eta_{dot} = 0$:

$$\left[g^A_{x,x}(\omega, 0)\right]^{-1} - \left[g^R_{x,x}(\omega, 0)\right]^{-1} \equiv 0. \quad (46)$$

The (correct) currents in the limit $\eta_{dot} = 0^+$ is thus different from the (incorrect) one for $\eta_{dot} = 0$. (All calculations in Refs. 1,2 are made with $\eta_{dot} = 0$, not with $\eta_{dot} = 0^+$, however in the different situation of a quantum dot with a resonant single-level for which adiabatic theorem could be demonstrated in Secs. I and II of this Supplemental Material). This result is obtained only for a specific toy-model of limited realism. This shows that, in general, $\eta_{dot} = 0$ or $\eta_{dot} = 0^+$ should be handled with care, which explains the motivation behind the detailed calculations presented in the previous sections of this Supplemental Material. Now, we come back to a single energy level at zero energy.

## III. A SECOND THEOREM: PRINCIPLE OF THE CODE FOR $\eta_{dot} \neq 0$

Introducing a finite value for the Dynes parameter $\eta_{dot}$ requires solving issues related to current conservation. It is as if the quantum dot with continuous spectrum would play the role of a fourth terminal being a source or a sink of current and thus, its chemical potential has to be specified. It is indeed demonstrated that *the bare populations of the quantum dot (those at time $t = -\infty$ in adiabatic procedure) have to be calculated self-consistently in such a way as to impose current conservation in the fully dressed steady state.* This means introduction of a self-consistency loop on those bare populations in order to enforce current conservation.

It is demonstrated now that the procedure discussed in Ref. 7 is equivalent to the statement above on the determination of the bare populations, calculated in such a way as to enforce current conservation in the steady state. The case of normal electrodes is considered first in Sec. III A, and those calculations are extended next to the superconducting case in Sec. III B. In both cases, the calculations are carried out to all orders, thus generalizing Ref. 7 which is focussed only on lowest order.

### A. Normal case

Appendix B in Ref. 7 is generalized, first by going to infinite order for normal metals (thus beyond lowest order). Current conservation in the steady state is automatically fulfilled once the divergences have been "removed" with this procedure.

#### 1. Expression of the Keldysh Green's function

The quantum dot Green's function corresponds to one level at zero energy [see Eq. (4)]. The quantum dot Keldysh Green's function is given by

$$G^{+,-}_{x,x} = \left(1 + G^R\Sigma\right)_{x,x} g^{+,-}_{x,x} \left(1 + \Sigma G^A\right)_{x,x} + \sum_k \left(1 + G^R\Sigma\right)_{x,k} g^{+,-}_{k,k} \left(1 + \Sigma G^A\right)_{k,x} . \tag{47}$$

Using the identity $G^{A,R}_{x,x} = \left(1 + g^{A,R}_{x,x}\Gamma^A\right)^{-1} g^{A,R}_{x,x}$ leads to

$$G^{+,-}_{x,x} = \left(1 - g^R_{x,x}\Gamma^R\right)^{-1} \left[g^{+,-}_{x,x} + g^R_{x,x}\Gamma_{eff} g^A_{x,x}\right] \left(1 - \Gamma^A g^A_{x,x}\right)^{-1} , \tag{48}$$

where $\Gamma^{A,R}$ are given by

$$\Gamma^{A,R} = \Sigma_{x,a} g^{A,R}_{a,a} \Sigma_{a,x} + \Sigma_{x,b} g^{A,R}_{b,b} \Sigma_{b,x} + \Sigma_{x,c} g^{A,R}_{c,c} \Sigma_{c,x} . \tag{49}$$

The parameter $\Gamma_{eff}$ in Eq. (48) contains the Keldysh Green's function:

$$\Gamma_{eff} = \Sigma_{x,a} g^{+,-}_{a,a} \Sigma_{a,x} + \Sigma_{x,b} g^{+,-}_{b,b} \Sigma_{b,x} + \Sigma_{x,c} g^{+,-}_{c,c} \Sigma_{c,x} . \tag{50}$$

The Keldysh Green's function is expanded in powers of $\Gamma/\eta_{dot}$:

$$\hat{g}^{+,-} = \sum_p \hat{g}^{+,-(p)}, \tag{51}$$

where $\hat{g}^{+,-(p)} \sim (\Gamma/\eta_{dot})^p$ takes the following form: $\hat{g}^{+,-(p)}(\omega) = \hat{n}^{(p)}(\omega) \left[\hat{g}^A(\omega) - \hat{g}^R(\omega)\right]$.

#### 2. Populations to order zero and connection with Ref. 7

The populations are first calculated to order zero in the tunnel amplitudes coupling the dot to the normal reservoirs ($p = \alpha = 0$). The Keldysh Green's function $G^{+,-}_{x,x}$ is expanded to order two in the tunnel amplitudes:

$$G^{+,-} = g^{+,-} + g^R\Gamma^R g^{+,-(0,0)} + g^{+,-(0,0)}\Gamma^A g^A + g^R\Gamma^{eff} g^A, \tag{52}$$

where the labels "$x,x$" are implicit. The superscript $(0,0)$ in $g^{+,-(0,0)}$ is used as a notation for $p=\alpha=0$. The following identity

$$\int d\omega \left\{ n^{(0)} \left( g^R\Gamma^R + g^A\Gamma^A \right) \left( g^A - g^R \right) + g^R\Gamma^{eff} g^A \right\} = 0 \tag{53}$$

implies a cancellation of divergences to lowest order, leading to

$$n^{(0)} = -\frac{\int d\omega g^R \Gamma^{eff} g^A}{\int d\omega \left( g^R\Gamma^R + g^A\Gamma^A \right) \left( g^A - g^R \right)}. \tag{54}$$

The numerator and the denominator are both of order $\Gamma/\eta_{dot}$, meaning that, indeed, the populations are calculated to order zero. Eq. (B7) of Ref. 7 is recovered.

### *3. Recursions at arbitrary order*

Cancelling the divergences term by term leads to

$$\begin{aligned} 2i\pi n^{(p)}(0) &= -\int d\omega \sum_{p_1,q_1} \sum_{n_1=0}^{+\infty} \delta_{p,p_1+q_1+n_1} (\Gamma)^{p_1+q_1} (g^A_{x,x})^{p_1} (g^R_{x,x})^{q_1} \times 2i\pi n^{(n_1)}(0)\delta(\omega) \\ &- \int d\omega \sum_{p_2,q_2} \delta_{p,p_2+q_2} (\Gamma)^{p_2+q_2} (g^A_{x,x})^{p_2} (g^R_{x,x})^{q_2} |g_{x,x}|^2 \Gamma_{eff}. \end{aligned} \tag{55}$$

"Renormalizing" all terms leads to

$$\int d\omega G^{+,-}_{x,x}(\omega) = \int d\omega g^{+,-}_{x,x}(\omega) = 2i\pi \sum_{p=0}^{+\infty} n^{(p)}. \tag{56}$$

Carrying out the summation over $p$ in Eq. (55) leads to

$$g^{+,-}_{x,x} = \left(1-\Gamma g^R_{x,x}\right)^{-1} g^{+,-}_{x,x} \left(1-\Gamma g^A_{x,x}\right)^{-1} + \left(1-\Gamma g^R_{x,x}\right)^{-1} g^R_{x,x} \Gamma_{eff} g^A_{x,x} \left(1-\Gamma g^A_{x,x}\right)^{-1}. \tag{57}$$

It is deduced that

$$\Gamma_{eff} = -\Gamma^R g^{+,-}_{x,x} (g^A_{x,x})^{-1} - (g^R_{x,x})^{-1} g^{+,-}_{x,x} \Gamma^A + \Gamma^R g^{+,-}_{x,x} \Gamma^A. \tag{58}$$

However, $\Gamma^R g^{+,-}_{x,x} (g^A_{x,x})^{-1}$ and $(g^R_{x,x})^{-1} g^{+,-}_{x,x} \Gamma^A$ tend to zero in the limit $\eta_{dot} \to 0^+$ while $\Gamma^R g^{+,-}_{x,x} \Gamma^A$ tends to a $\delta$-function. It is thus deduced that

$$\Gamma_{eff} = \Gamma^R g^{+,-}_{x,x} \Gamma^A. \tag{59}$$

### *4. Equivalence to current conservation*

Starting from the expression of the current in terms of the Keldysh Green's functions, it can be shown that

$$\begin{aligned} I_{tot} &= \frac{e}{h} \int d\omega \sum_{\tau} \langle 0 | \Gamma^R \left( G^{+,-}_{x,x} - g^{+,-}_{x,x} \right) - \left( G^{+,-}_{x,x} - g^{+,-}_{x,x} \right) \Gamma^A \\ &+ \Gamma_{eff} G^A_{x,x} - G^R_{x,x} \Gamma_{eff} - \Gamma^R g^{+,-}_{x,x} \Gamma^A G^A_{x,x} + G^R_{x,x} \Gamma^R g^{+,-}_{x,x} \Gamma^A | 0 \rangle, \end{aligned} \tag{60}$$

where the state $|0\rangle$ has the meaning of the harmonics $n=0$ of half the Josephson frequency $n\omega_0/2$. The self-consistency equation $G^{+,-} = g^{+,-}$ leads to Eq. (59). Thus, extra terms have to be added at time $t=-\infty$ to the bare Hamiltonian, corresponding to those bare quantum dot populations at time $t=-\infty$, calculated in such a way that current conservation is fulfilled in the steady state. This discussion resembles the calculation for the Fermi surface in strongly correlated systems[8].

## B. Superconducting case

The generalization to the superconducting case is presented below. The same equivalence between Ref. 7 and current conservation in the steady state is obtained, which provides the principle of the numerical code for finite $\eta_{dot}/\Delta$ (see also the beginning of Sec. III A in Supplemental Material).

### 1. Expression of the Keldysh Green's function

The fully dressed Green's function of the quantum dot has an expression analogous to its normal state counterpart [see Eq. (48)], the Green's function being now a matrix in Nambu and in the space of harmonics of half the Josephson frequency.

In the superconducting case, the Keldysh Green's function is expanded in powers of $1/\eta_{dot}$, but also in powers of $\Gamma$:

$$\hat{g}^{+,-} = \sum_{p,\alpha} \hat{g}^{+,-(p,\alpha)}, \tag{61}$$

with $\hat{g}^{+,-(p,\alpha)}$ behaving like $\hat{g}^{+,-(p,\alpha)} \sim \Gamma^p \eta_{dot}^{-\alpha}$ in the small-$\Gamma$ and small-$\eta_{dot}$ limits.

### 2. Construction of the recursion

The calculation proceeds by evaluating $\hat{g}^{+,-}$ order by order in such a way as to cancel all divergences in $\hat{G}^{+,-}$. In the end of the recursion, the Keldysh Green's function is "renormalized" into $\hat{g}^{+,-}$, which has a simple structure in energy: it is made of $\delta$-peaks at harmonics of the Josephson frequency, which account for the weight of those resonances, however without containing information about their width in energy.

Now, the calculation for the populations is generalized to arbitrary order, in the superconducting case:

$$\hat{G}^{+,-}(\omega \approx n_0\omega_0/2) = \sum_{K,\gamma} \left\{ \hat{G}_A^{+,-(K,\gamma)}(\omega \approx n_0\omega_0/2) + \hat{G}_B^{+,-(K,\gamma)}(\omega \approx n_0\omega_0/2) \right\}, \tag{62}$$

with

$$\hat{G}_A^{+,-}(\omega \approx n_0\omega_0/2) = \left(\hat{I} - \hat{g}^R\hat{\Gamma}^R\right)^{-1} \hat{g}^{+,-}_{x,x} \left(\hat{I} - \hat{\Gamma}^A\hat{g}^A_{x,x}\right)^{-1} = \sum_{n,m\geq 0} \left(\hat{g}^R\hat{\Gamma}^R\right)^n \hat{g}^{+,-} \left(\hat{\Gamma}^A\hat{g}^A\right)^m, \tag{63}$$

and

$$\hat{G}_B^{+,-}(\omega \approx n_0\omega_0/2) = \left(\hat{I} - \hat{g}^R\hat{\Gamma}^R\right)^{-1} \left[\hat{g}^R_{x,x}\hat{\Gamma}_{eff}\hat{g}^A_{x,x}\right] \left(\hat{I} - \hat{\Gamma}^A\hat{g}^A_{x,x}\right)^{-1} \tag{64}$$

$$= \sum_{n,m\geq 0} \left(\hat{g}^R\hat{\Gamma}^R\right)^n \hat{g}^R\hat{\Gamma}^{eff}\hat{g}^A \left(\hat{\Gamma}^A\hat{g}^A\right)^m, \tag{65}$$

where the label "$x, x$" is implicit. The strategy of the forthcoming calculation is to start from Eqs. (63)-(65), and to expand those equations in series of $K$ and $\gamma$, as in Eq. (62).

First, using Eq. (51) leads to an expansion of $\hat{G}_A^{+,-}(\omega \approx n_0\omega_0/2)$ and $\hat{G}_B^{+,-}(\omega \approx n_0\omega_0/2)$ as a series containing terms of order $K$ in $\Gamma$. The series in $\gamma$ is treated next. Eq. (63) becomes: $\hat{G}_A^{+,-}(\omega \approx n_0\omega_0/2) = \sum_{K,\gamma} \hat{G}_A^{+,-(K,\gamma)}(\omega \approx n_0\omega_0/2)$, with

$$\hat{G}_A^{+,-(K,\gamma)}(\omega \approx n_0\omega_0/2) = \sum_{\alpha,\beta} \sum_{n,m,p\geq 0} \sum_{\{\tau_q,N_q\}} \delta_{\alpha+\beta,\gamma}\delta_{K,p+n+m} \tag{66}$$

$$\times \left( \prod_{i=0}^{n-1} \langle \tau_i, N_i | \hat{g}^R\hat{\Gamma}^R | \tau_{i+1}, N_{i+1} \rangle \right) \langle \tau_n, N_n | \hat{g}^{+,-(p,\alpha)} | \tau_{n+1}, N_{n+1} \rangle$$

$$\times \left( \prod_{j=n+1}^{n+m} \langle \tau_j, N_j | \hat{\Gamma}^A\hat{g}^A | \tau_{j+1}, N_{j+1} \rangle \right) \delta_{\tau_0,1}\delta_{N_0,0}\delta_{\tau_{n+m+1},1}\delta_{N_{n+m+1},0}\delta_{\beta,F_{n_0}[N_k]},$$

where the Keldysh Green's function is evaluated at $\omega \approx n_0\omega_0/2$. In analogy with the fictitious 1D tight-binding Hamiltonian of a single $S_a - S_b$ contact[6], the notation $|\tau_k, N_k\rangle$ stands for a fictitious quantum state with Nambu label $\tau_k$ and harmonics label $N_k$. The degree of a singularity at $\omega = n_0\omega_0/2$ is given by

$$F_{n_0}[N_k] = \sum_{k=0}^{n-1} \delta_{n_0+N_k,0} + \sum_{k=n+2}^{n+m+1} \delta_{n_0+N_k,0}, \tag{67}$$

Applying the same treatment to $\hat{G}_B^{+,-(K,\gamma)}(\omega \approx n_0\omega_0/2)$ in Eqs. (64)-(65) leads to $\hat{G}_B^{+,-}(\omega \approx n_0\omega_0/2) = \sum_{K',\gamma'} \hat{G}_B^{+,-(K',\gamma')}(\omega \approx n_0\omega_0/2)$, with

$$\begin{aligned}
\hat{G}_B^{+,-(K',\gamma')}(\omega \approx n_0\omega_0/2) &= \sum_{n',m'} \sum_{\{\tau'_{q'},N'_{q'}\}} \delta_{\alpha+\beta,\gamma}\delta_{K,p'+n'+m'} \\
&\times \left( \prod_{i'=0}^{n'-1} \langle \tau'_{i'}, N'_{i'} | \hat{g}^R \hat{\Gamma}^R | \tau'_{i'+1}, N'_{i'+1} \rangle \right) \langle \tau'_{n'}, N'_{n'} | \hat{g}^R | \tau'_{n'+1}, N'_{n'+1} \rangle \\
&\times \langle \tau'_{n'+1}, N'_{n'+1} | \hat{\Gamma}^{eff} | \tau'_{n'+2}, N'_{n'+2} \rangle \langle \tau'_{n'+2}, N'_{n'+2} | \hat{g}^A | \tau'_{n'+3}, N'_{n'+3} \rangle \\
&\times \left( \prod_{j'=n'+3}^{n'+m'+2} \langle \tau'_{j'}, N'_{j'} | \hat{\Gamma}^A \hat{g}^A | \tau'_{j'+1}, N'_{j'+1} \rangle \right) \delta_{\tau'_0,1}\delta_{N'_0,0}\delta_{\tau'_{n'+m'+3},0}\delta_{N'_{n'+m'+3},0}\delta_{\gamma',-1+F'_{n_0}[N'_{k'}]},
\end{aligned} \tag{68}$$

with

$$F'_{n_0}[N_{k'}] = \sum_{k'=0}^{n'} \delta_{n_0+N'_{k'},0} + \sum_{k'=n'+3}^{n'+m'+3} \delta_{n_0+N'_{k'},0}. \tag{69}$$

Next, the following set of equations is solved by recursion:

$$\int_{n_0\omega_0/2-\epsilon}^{n_0\omega_0/2+\epsilon} \left\{ \hat{G}_A^{+,-(K,\gamma)}(\omega) + \hat{G}_B^{+,-(K,\gamma)}(\omega) \right\} = 0, \tag{70}$$

where $\epsilon$ is taken around $\epsilon \simeq \omega_0/4$. First Eq. (70) is considered for $\gamma = 0$, leading to the expression of $\hat{g}^{+,-(K,0)}$ as a function of $\hat{g}^{+,-(p,0)}$ with $p < K$, which can be recast as a recursion for the occupation numbers:

$$\hat{n}^{(K,0)} = \mathcal{F} \left\{ \hat{n}^{(p,0)} \right\}_{p<K}, \tag{71}$$

where the function $\mathcal{F}$ is deduced in a straightforward manner from Eqs. (66), (68) and (70).

Considering next $\gamma = 1$, then it is possible to show that $\hat{g}^{+,-(K,1)}$ is a function of $\hat{g}^{+,-(p,0)}$ for $p \leq K$ and, $\hat{g}^{+,-(q,1)}$ for $q < K$, with the corresponding recursion for the occupation numbers:

$$\hat{n}^{(K,1)} = \mathcal{G} \left\{ \left[ \hat{n}^{(p,0)} \right]_{p \leq K}, \left[ \hat{n}^{(p,1)} \right]_{p<K} \right\}. \tag{72}$$

Similar recursions allow to calculate all of the $\hat{n}^{(K,\alpha)}$s.

#### 3. *Equivalence to current conservation*

It is then easy to sum over $(K,\gamma)$ and $(K',\gamma')$ is Eqs. (66) and (68) to show that current conservation is automatically fulfilled. The demonstration for this last step follows Sec. III A 4 above in the normal case.

## IV. FAILURE OF THE KELDYSH ALGORITHM IN THE PRESENCE OF A DISCRETE SPECTRUM

The adiabatic theorem was demonstrated (see Secs. I and II in Supplemental Material above) only for a continuous spectrum [See the parameter $\gamma_0$ in Eq. (18)]. However, *the Keldysh procedure fails to produce the correct dressed*

*density matrix in the case of a discrete spectrum.* This statement is especially interesting, in view of the exponential smallness in $\Delta/eV$ of the processes equilibrating the quantum dot degrees of freedom and the half-infinite quasiparticle continua above the gaps. This justifies the introduction of Dynes parameters in the numerical calculations, which, in addition of being physically motivated, have the effect of making the FLS spectra become continuous.

The starting point is $H = H_0 + V$, with $H|i\rangle = \epsilon_i|i\rangle$. In the adiabatic switching procedure, we use $H(t) = H_0 + \exp(\eta t)V$ for $-\infty < t < 0$ and with $\eta \to 0^+$. The system evolution is considered in the adiabatic picture:

$$i\frac{d}{dt}|\psi(t)\rangle = \exp(\eta t)\exp(iH_0 t)V\exp(-iH_0 t)|\psi(t)\rangle. \tag{73}$$

The system is assumed to be in the eigenstate $|0\rangle$ of $H_0$ in the limit $t \to -\infty$. The dressed state corresponding to $|0\rangle$ is

$$U_\eta(0,-\infty)|0\rangle = \sum_{n=0}^{+\infty}(-i)^n\int_{-\infty}^{0}dt_1...\int_{-\infty}^{t_{n-1}}dt_n e^{\eta(t_1+...+t_n)}V_I(t_1)...V_I(t_n)|0\rangle \tag{74}$$

$$= \sum_{n=0}^{+\infty}\sum_{i_1,...,i_n}(-i)^n\int_{-\infty}^{0}dt_1\int_{-\infty}^{t_1}dt_2...\int_{-\infty}^{t_{n-1}}dt_n \tag{75}$$
$$\times \exp\left\{\eta(t_1+...+t_n) + i\left[(\epsilon_{i_1}-\epsilon_{i_2})t_1 + ... + (\epsilon_{i_n}-\epsilon_0)t_n\right]\right\} V_{i_1,i_2}...V_{i_n,0}|i_1\rangle.$$

To compute the integral, it is convenient to change variables according to $t_1 = -\tau_1$, $t_2 = -\tau_1 - \tau_2$, ..., $t_n = -\tau_1 - \tau_2 - ... - \tau_n$. Then:

$$t_1 + t_2 + .... + t_n = -\left[n\tau_1 + (n-1)\tau_2 + ... + 2\tau_{n-1} + \tau_n\right] \tag{76}$$

and the phase factor in Eq. (75) is

$$(\epsilon_0 - \epsilon_1)\tau_1 + (\epsilon_0 - \epsilon_{i_1})\tau_2 + ... + (\epsilon_0 - \epsilon_{i_n})\tau_n, \tag{77}$$

leading to

$$U_\eta(0,-\infty)|0\rangle = \sum_{n=0}^{+\infty}\frac{1}{\epsilon_0 - H_0 + in\eta}V\frac{1}{\epsilon_0 - H_0 + i(n-1)\eta}V...V\frac{1}{\epsilon_0 - H_0 + i\eta}V|0\rangle. \tag{78}$$

The adiabatic theorem states that $\lim_{\eta\to 0^+} U_\eta(0,-\infty)|0\rangle$ is proportional to an eigenstate of $H = H_0 + V$ [under non-degeneracy assumptions on the spectrum of $H_0 + \lambda V$]. However, the relatively complicated pattern of imaginary parts makes an exact evaluation of Eq. (78) difficult.

In many-body systems, a common practise is to exchange the $n \to +\infty$ and the $\eta \to 0^+$ limits. However, interchanging limits is problematic in the case of a discrete spectrum, but this exchange of limits is expected to be valid for a continuous spectrum, where it is closely related to the Lippmann-Schwinger equations for steady states in the presence of a scattering potential. Making the inversion of limits leads to

$$U_\eta^{(K)}|0\rangle = \sum_{n=0}^{+\infty}G_0(\epsilon_0)VG_0(\epsilon_0)...G_0(\epsilon_0)V|0\rangle = \sum_{n=0}^{+\infty}\left(G(\epsilon_0)V\right)^n|0\rangle, \tag{79}$$

where $G_0(\omega)$ is the "bare" retarded propagator $G_0(\omega) = 1/(\omega - H_0 + i\eta)$. Denoting the l.h.s. by $|0,V\rangle$, it satisfies the equation

$$|0,V\rangle = |0\rangle + G_0(\epsilon_0)V|0,V\rangle \tag{80}$$

which is known as the Lippmann-Schwinger equation [see also Sec. V above]. Multiplying Eq. (80) by $\epsilon_0 - H_0 + i\eta$ leads to

$$\left(\epsilon_0 - H_0 - V + i\eta\right)|0,V\rangle = \left(\epsilon_0 - H_0 + i\eta\right)|0\rangle = i\eta|0\rangle. \tag{81}$$

Using the spectral decomposition of $H$: $H|\alpha\rangle = E_\alpha|\alpha\rangle$, we can write

$$|0,V\rangle = \sum_\alpha |\alpha\rangle\frac{i\eta}{\epsilon_0 - E_\alpha + i\eta}\langle\alpha|0\rangle. \tag{82}$$

Three remarks are in order:

1. If the spectrum is discrete and if $E_\alpha \neq \epsilon_0$ for all $\alpha$, then $\lim_{\eta\to 0^+} |0, V\rangle = 0$, signaling a failure of this procedure.

2. If the spectrum is discrete and $E_\alpha = \epsilon_0$ for one $\alpha$, then $\lim_{\eta\to 0^+} |0, V\rangle = 0 = \langle\alpha|0\rangle|\alpha\rangle$. A dressed state as desired. However $|\langle\alpha|0\rangle| < 1$ in general and the adiabatic evolution is not unitary.

3. If $\epsilon_0$ belongs to an interval in which the spectrum of $H$ is continuous, then an exact eigenstate of $H_0 + V$ with the same eigenvalue $\epsilon_0$ is expected to be obtained.

An intermediate situation is obtained for a three-terminal Josephson junction, because of the Floquet-Wannier-Stark states inside the gap. In this case, the Keldysh algorithm can be made operational (see Secs. I and II in Supplemental Material), once supplemented with self-consistency on the initial condition on the quantum dot bare populations.

## V. FLOQUET-LIPPMANN-SCHWINGER DRESSING ALGORITHM

This section presents calculations for the Floquet-Lippmann-Schwinger algorithm. The method shares similarities with the Floquet scattering approach[9–13]. The Bogoliubov-de Gennes equations are obtained first, and Floquet-Lippmann-Schwinger calculations are presented next. No difficulty arises with current conservation. Those calculations are the basis for the Floquet-Lippmann-Schwinger wave-function calculation presented in the paper, in Fig. 7b.

### A. Bogoliubov-de Gennes equations

The time-dependent Bogoliubov-de Gennes equations are interpreted as a single particle Hamiltonian evolution in Nambu space, and Floquet theory can be applied. If $U(t)$ is the evolution operator [with $\mathcal{H}(t)$ given by Eqs. (A1)-(A3); see Appendix A in the paper], we define

$$\gamma^+(t) = U(t)\gamma^+(0)U(t)^{-1}. \tag{83}$$

The operator $\gamma^+(t)$ in Eq. (83) is*not* the Heisenberg picture $\gamma^+_H(t) = U(t)^{-1}\gamma^+(0)U(t)$. With Eq. (83), the Bogoliubov-de Gennes equations take the form

$$i\frac{d}{dt}\gamma^+(t) = \left[H(t), \gamma^+(t)\right]. \tag{84}$$

On the other hand, for Heisenberg operators, we have

$$i\frac{d}{dt}\gamma^+_H(t) = \left[\gamma^+_H(t), \mathcal{H}_H(t)\right]. \tag{85}$$

Eq. (84) seems easier to solve than Eq. (85), because we can expand $\gamma^+(t)$ in the basis of time-independent fermionic creation and annihilation operators. A first-order differential equation will be obtained for the evolution of the components of $\gamma^+(t)$. But for Eq. (85), we would meet the difficulty that $\mathcal{H}_H(t)$ is not known.

The operator $\gamma^+(t)$ is written as

$$\gamma^+(t) = u(t)d^+_\uparrow + v(t)d_\downarrow + \sum_{j,\mathbf{k}} u_{j,\mathbf{k}}(t)c^+_{j,\mathbf{k},\uparrow} + v_{j,\mathbf{k}}(t)c_{j,-\mathbf{k},\downarrow}. \tag{86}$$

Taking into account the following commutators

$$\left[\mathcal{H}(t), d^+_\uparrow\right] = \sum_{j,\mathbf{k}} J_{j,\mathbf{k}} e^{-i\omega_j t} c^+_{j,\mathbf{k},\uparrow} \tag{87}$$

$$\left[\mathcal{H}(t), d_\downarrow\right] = -\sum_{j,\mathbf{k}} J_{j,\mathbf{k}} e^{i\omega_j t} c^+_{j,-\mathbf{k},\uparrow} \tag{88}$$

$$\left[\mathcal{H}(t), c^+_{j,\mathbf{k},\uparrow}\right] = J_{j,\mathbf{k}} e^{i\omega_j t} d^+_\uparrow + \epsilon_{\mathbf{k}} c^+_{j,\mathbf{k},\uparrow} + \Delta^*_j c_{j,-\mathbf{k},\downarrow} \tag{89}$$

$$\left[\mathcal{H}(t), c_{j,-\mathbf{k},\downarrow}\right] = -J_{j,\mathbf{k}} e^{-i\omega_j t} d_\downarrow + \Delta_j c^+_{j,\mathbf{k},\uparrow} - \epsilon_{\mathbf{k}} c_{j,-\mathbf{k},\downarrow} \tag{90}$$

leads to the Bogoliubov-de Gennes equations

$$\frac{d}{dt}u(t) = \sum_{j,\mathbf{k}} J_{j,\mathbf{k}} e^{i\omega_j t} u_{j,\mathbf{k}}(t) \tag{91}$$

$$\frac{d}{dt}v(t) = -\sum_{j,\mathbf{k}} J_{j,\mathbf{k}} e^{-i\omega_j t} v_{j,\mathbf{k}}(t) \tag{92}$$

$$\frac{d}{dt}u_{j,\mathbf{k}}(t) = \epsilon_{\mathbf{k}} u_{j,\mathbf{k}}(t) + \Delta_j v_{j,\mathbf{k}}(t) + J_{j,\mathbf{k}} e^{-i\omega_j t} u(t) \tag{93}$$

$$\frac{d}{dt}v_{j,\mathbf{k}}(t) = \Delta_j^* u_{j,\mathbf{k}}(t) - \epsilon_{\mathbf{k}} v_{j,\mathbf{k}}(t) - J_{j,\mathbf{k}} e^{i\omega_j t} v(t). \tag{94}$$

Specializing now to a commensurate configuration of voltages, we have $\omega_j = s_j\omega$, with $s_j$ an integer. For instance, for the three-terminal configuration of interest, $s_j \in \{\pm 1, 0\}$ in the quartet configuration. The Floquet eigenvectors take the form

$$u(t) = e^{-iEt} \sum_m e^{-im\omega_0 t} u(m) \tag{95}$$

$$u_{j,\mathbf{k}}(t) = e^{-iEt} \sum_m e^{-im\omega_0 t} u_{j,k}(m), \tag{96}$$

and so on. Extracting the Fourier components in the Bogoliubov-de Gennes equations leads to

$$(E + m\omega_0) u(m) = \sum_{j,\mathbf{k}} J_{j,\mathbf{k}} u_{j,\mathbf{k}}(m + s_j) \tag{97}$$

$$(E + m\omega_0) v(m) = -\sum_{j,\mathbf{k}} J_{j,\mathbf{k}} v_{j,\mathbf{k}}(m - s_j) \tag{98}$$

$$(E + m\omega_0) u_{j,\mathbf{k}}(m) = \epsilon_{\mathbf{k}} u_{j,\mathbf{k}}(m) + \Delta_j v_{j,\mathbf{k}}(m) + J_{j,\mathbf{k}} u(m - s_j) \tag{99}$$

$$(E + m\omega_0) v_{j,\mathbf{k}}(m) = \Delta_j^* u_{j,\mathbf{k}}(m) - \epsilon_{\mathbf{k}} v_{j,\mathbf{k}}(m) - J_{j,\mathbf{k}} v(m + s_j). \tag{100}$$

The amplitudes $(u_{j,\mathbf{k}}(m), v_{j,\mathbf{k}}(m))$ associated to the reservoirs can be eliminated:

$$\begin{pmatrix} u_{j,\mathbf{k}}(m) \\ v_{j,\mathbf{k}}(m) \end{pmatrix} = \frac{J_{j,\mathbf{k}}}{(E + m\omega_0)^2 - \epsilon_{\mathbf{k}}^2 - |\Delta_j|^2} \begin{pmatrix} E + m\omega_0 + \epsilon_{\mathbf{k}} & \Delta_j \\ \Delta_j^* & E + m\omega_0 - \epsilon_{\mathbf{k}} \end{pmatrix} \begin{pmatrix} u(m - s_j) \\ -v(m + s_j) \end{pmatrix}. \tag{101}$$

To put back those amplitudes in the equations for $u(m)$ and $v(m)$, it is first required to evaluate

$$u_{j,\mathbf{k}}(m + s_j) = \frac{J_{j,\mathbf{k}}}{(E + (m + s_j)\omega_0)^2 - \epsilon_{\mathbf{k}}^2 - |\Delta_j|^2} \left[ \left( E + (m + s_j)\omega_0 + \epsilon_{\mathbf{k}} \right) u(m) - \Delta_j v(m + 2s_j) \right] \tag{102}$$

$$v_{j,\mathbf{k}}(m - s_j) = \frac{J_{j,\mathbf{k}}}{(E + (m - s_j)\omega_0)^2 - \epsilon_{\mathbf{k}}^2 - |\Delta_j|^2} \left[ \Delta_j^* u(m - 2s_j) - \left( E + (m - s_j)\omega_0 - \epsilon_{\mathbf{k}} \right) v(m) \right], \tag{103}$$

leading to

$$\left( E + m\omega_0 - \sum_{j,\mathbf{k}} J_{j,\mathbf{k}}^2 \frac{E + (m + s_j)\omega_0 + \epsilon_{\mathbf{k}}}{(E + (m + s_j)\omega_0)^2 - \epsilon_{\mathbf{k}}^2 - |\Delta_j|^2} \right) u(m) \tag{104}$$
$$+ \sum_{j,\mathbf{k}} \frac{J_{j,\mathbf{k}}^2 \Delta_j}{(E + (m + s_j)\omega_0)^2 - \epsilon_{\mathbf{k}}^2 - |\Delta_j|^2} v(m + 2s_j) = 0$$

$$\sum_{j,\mathbf{k}} \frac{J_{j,\mathbf{k}}^2 \Delta_j^*}{(E + (m - s_j\omega_0)^2 - \epsilon_{\mathbf{k}}^2 - |\Delta_j|^2} u(m - 2s_j) \tag{105}$$
$$+ \left( E + m\omega_0 - \sum_{j,\mathbf{k}} J_{j,\mathbf{k}}^2 \frac{E + (m - s_j)\omega_0 - \epsilon_{\mathbf{k}}}{(E + (m - s_j)\omega_0)^2 - \epsilon_{\mathbf{k}}^2 - |\Delta_j|^2} \right) v(m) = 0$$

The off-diagonal terms connecting the $u$'s and $v$'s correspond to Andreev reflection processes. Besides numerics, those equations may be analyzed in two ways: perturbation theory in the off-diagonal terms, if transmissions at the interfaces between the dot and the leads are small, or semi-classics if $\omega_0 \to 0$. The solution of a similar system of equations is presented in Ref. 14.

### B. Floquet-Lippmann-Schwinger dressing algorithm

A Floquet solution of Eq. (84) is $\gamma^+_E(t)$, such that $\gamma^+_E(t+T)=\exp(-iET)\gamma_E(t)$, with $T=2\pi/\omega_0$. The Lippmann-Schwinger approach amounts to construct this Floquet basis, starting from eigenstates in the leads, which form a continuous spectrum:

$$\gamma^{+(0)}_{l,\mathbf{k},\sigma}(t)=e^{-iE_{l,\mathbf{k}}t}\left(x_{l,\mathbf{k}}e^{i\varphi_l/2}c^+_{l,\mathbf{k},\sigma}+\sigma y_{l,\mathbf{k}}e^{-i\varphi_l/2}c_{l,-\mathbf{k},-\sigma}\right), \tag{106}$$

where $l$ denotes the reservoir [as in Eqs. (A1)-(A3) of Appendix A in the paper], $E_{l,\mathbf{k}}=\left(\epsilon^2_{\mathbf{k}}+|\Delta_l|^2\right)^{1/2}$, and $\sigma=\pm$ is the spin component along $\hat{z}$ axis. In Eq. (106), the coefficients $x_{l,\mathbf{k}}$ and $y_{l,\mathbf{k}}$ are given by

$$x_{l,\mathbf{k}}=\frac{\sqrt{\sqrt{\epsilon^2_{\mathbf{k}}+|\Delta_l|^2}+\epsilon_{\mathbf{k}}}}{\sqrt{2}\left(\epsilon^2_{\mathbf{k}}+|\Delta_l|^2\right)^{1/4}}\text{and } y_{l,\mathbf{k}}=\frac{\sqrt{\sqrt{\epsilon^2_{\mathbf{k}}+|\Delta_l|^2}-\epsilon_{\mathbf{k}}}}{\sqrt{2}\left(\epsilon^2_{\mathbf{k}}+|\Delta_l|^2\right)^{1/4}}. \tag{107}$$

The dressed Floquet-Lippmann-Schwinger quasiparticle operator takes the form

$$\gamma^+_{l,\mathbf{k},\sigma}(t) = \gamma^{+(0)}_{l,\mathbf{k},\sigma}(t)+e^{-iE_{l,\mathbf{k}}t}\sum_m e^{-im\omega_0 t}\times \tag{108}$$

$$\left\{u_{l,\mathbf{k}}(m)d^+_\sigma+\sigma v_{l,\mathbf{k}}(m)d_{-\sigma}+\sum_{j,\mathbf{q}}\left(u_{j,\mathbf{q};l,\mathbf{k}}(m)c^+_{j,\mathbf{q},\sigma}+\sigma v_{j,\mathbf{q};l,\mathbf{k}}(m)c_{j,-\mathbf{q},-\sigma}\right)\right\}$$

The coefficients satisfy the following inhomogeneous equations (Lippmann-Schwinger in the enlarged single particle Hilbert space):

$$(E+m\omega_0+i\eta)u_{l,\mathbf{k}}(m) = J_{l,\mathbf{k}}\delta_{m,-s_l}x_{l,\mathbf{k}}e^{i\varphi_l/2}+\sum_{j,\mathbf{q}}J_{j,\mathbf{q}}u_{j,\mathbf{q};l,\mathbf{k}}(m+s_j) \tag{109}$$

$$(E+m\omega_0+i\eta)v_{l,\mathbf{k}}(m) = -J_{l,\mathbf{k}}\delta_{m,s_l}y_{l,\mathbf{k}}e^{-i\varphi_l/2}-\sum_{j,\mathbf{q}}J_{j,\mathbf{q}}v_{j,\mathbf{q};l,\mathbf{k}}(m-s_j), \tag{110}$$

and

$$(E+m\omega_0-\epsilon_{\mathbf{q}}+i\eta)u_{j,\mathbf{q};l,\mathbf{k}}(m) = \Delta_j v_{j,\mathbf{q};l,\mathbf{k}}(m)+J_{j,\mathbf{q}}u_{l,\mathbf{k}}(m-s_j) \tag{111}$$

$$(E+m\omega_0+\epsilon_{\mathbf{q}}+i\eta)v_{j,\mathbf{q};l,\mathbf{k}}(m) = \Delta^*_j u_{j,\mathbf{q};l,\mathbf{k}}(m)-J_{j,\mathbf{q}}v_{l,\mathbf{k}}(m+s_j). \tag{112}$$

Those equations were solved numerically by recursion in order to produce Fig. 5b.

## VI. TILTED BAND PICTURE AND FLOQUET-WANNIER-STARK VIEWPOINT

An introduction to the FWS viewpoint is provided in this Section. The ideas presented here are equivalent to Refs. 9,10. Simple situations are considered first, gradually making the description more complex and incorporating the realistic ingredients of three-terminal set-ups. The extended Hamiltonian is introduced in Sec. VI A in the context of classical mechanics with $\hbar=0$. Sec. VI B restores a finite $\hbar$ on a few examples. Sec. VI C deals with the extended Hamiltonian in the presence of a band structure, such as that provided by a single energy band. The FWS viewpoint of three-terminal Josephson junctions is presented in the main body of the paper (see the self-contained Sec. II in the paper).

### A. Classical mechanics

First getting rid of quantum mechanics, a classical Hamiltonian $\mathcal{H}$ with $N$ degrees of freedom $(p_i,q_i)_{1\le i\le N}$ is considered. The Hamiltonian $\mathcal{H}$ is supposed to depend on an external control parameter $\theta$, with $\theta(t)=\theta_0+\omega_0 t$. We have $\mathcal{H}(\theta+2\pi)=\mathcal{H}(\theta)$. For superconducting set-ups, the variable $\theta$ would be analogous to the superconducting phase $\varphi$, and the relation $d\theta/dt=\omega_0$ would correspond to one of the Josephson relations, with $\omega_0=2eV/\hbar$ the Josephson

frequency associated to voltage $V$. The classical Hamiltonian $\mathcal{H}$ is transformed into a time-independent Hamiltonian $\tilde{\mathcal{H}}$ at the cost of introducing an additional continuous degree of freedom $l$. The pair $(\theta, l)$ of conjugate variables has the meaning of a generalized momentum $\theta$ conjugate to the "position" $l$. Thus, a new Hamiltonian is defined:

$$\tilde{\mathcal{H}}(p_1, q_1, ..., p_N, q_N, \theta, l) = \mathcal{H}(p_1, q_1, ..., p_N, q_N) - \omega_0 l. \tag{113}$$

Hamilton's equation $\dot{\theta} = -\partial\tilde{H}/\partial l = \omega_0$ leads to $\theta(t) = \theta_0 + \omega_0 t$ whatever the initial condition.

From a physical point of view, the variable $l$ corresponds to a generalized position and the $-\omega_0 l$ term to a uniform electric field for this additional degree of freedom. Contrary to the evolution of $\theta$, the evolution of the position $l$ depends nontrivially on the dynamics of the $N$ "physical" degrees of freedom, because

$$\dot{l} = \frac{\partial\tilde{\mathcal{H}}}{\partial\theta}(p_1, q_1, ..., p_N, q_N, \theta). \tag{114}$$

The introduction of an auxiliary space is considered now for a quantum mechanical Hamiltonian.

### B. Quantum mechanics

It is supposed that $|\theta\rangle = |\theta + 2\pi\rangle$ ($\theta$ playing the role of a momentum) because the Hamiltonian $\mathcal{H}(\theta)$ is $2\pi$-periodic in $\theta$. The interval $[0, 2\pi]$ is seen as the Brillouin zone for a 1D tight-binding Hamiltonian for the "position" $l$ (being now an integer). The vectors $|l\rangle$ are taken as an orthonormal basis of the space of the auxiliary variable.

The following relations hold: $\hat{l} = i\partial/\partial\theta$, and $\langle\theta|l\rangle = \exp(-il\theta)$, in analogy to (position,momentum) in quantum mechanics. Thus, $\hat{l}|l\rangle = l|l\rangle$.

It is useful to expand $\hat{\mathcal{H}}(\hat{\theta})$ in Fourier series:

$$\hat{\mathcal{H}} = \sum_n \hat{\mathcal{H}}_n \exp\left(-in\hat{\theta}\right), \tag{115}$$

where $\hat{\mathcal{H}}_n$ acts in the Hilbert space of the "physical" degrees of freedom.

It is then noted that

$$\exp\left(-in\hat{\theta}\right)|l\rangle = |l + n\rangle, \tag{116}$$

defining a translation operator. Then, the Hamiltonian takes the form

$$\hat{\mathcal{H}} = \sum_{l,n} \hat{\mathcal{H}}_n \otimes |l + n\rangle\langle l|. \tag{117}$$

This is a periodic Hamiltonian (from the point of view of the coordinate $l$), and $\hat{\mathcal{H}}_n$ plays the role of an "internal" Hamiltonian (like a generalized spin).

The corresponding Bloch state is obtained by fixing the generalized momentum $\theta$:

$$|\theta\rangle = \sum_l \exp(il\theta)|l\rangle. \tag{118}$$

Using the notation $|\psi\rangle = |\chi\rangle \otimes |\theta\rangle$, we have

$$\hat{\mathcal{H}}|\psi\rangle \; = \; \hat{\mathcal{H}}\left[|\chi\rangle \otimes |\theta\rangle\right] = \left(\hat{\mathcal{H}}(\theta)|\chi\rangle\right) \otimes |\theta\rangle. \tag{119}$$

The tilted band structure for the extended Hamiltonian is to be put in correspondence with the rotating basis $|\chi_n(\theta)\rangle$:

$$\hat{H}(\theta)|\chi_n(\theta)\rangle = E_n(\theta)|\chi_n(\theta)\rangle. \tag{120}$$

It is shown now that the generalized vector state is compatible with Schrödinger equation. At time $t = 0$, the state is $|\psi(t = 0)\rangle = |\chi(0)\rangle \otimes |\theta_0\rangle$. Then the solution of Schrödinger equation for the extended Hamiltonian $\hat{\mathcal{H}}(\theta) - \omega_0\hat{l}$ is (for all time $t$):

$$|\psi(t)\rangle = |\chi(t)\rangle \otimes |\theta_0 + \omega_0 t\rangle, \tag{121}$$

where $\chi(t)\rangle$ is the solution of the Schrödinger equation for the time-dependent Hamiltonian for the physical system:

$$i\frac{\partial}{\partial t}|\chi(t)\rangle = \mathcal{H}(\theta_0+\omega_0 t)|\chi(t)\rangle. \tag{122}$$

The demonstration is the following:

$$i\frac{d}{dt}|\theta_0+\omega_0 t\rangle = i\frac{d}{dt}\sum_l e^{il(\theta_0+\omega_0 t)}|l\rangle = \sum_l -\omega_0 l e^{il(\theta_0+\omega_0 t)}|l\rangle = -\omega_0\hat{l}|\theta_0+\omega_0 t\rangle. \tag{123}$$

Let us suppose that Eq. (122) is verified. Then:

$$i\frac{d}{dt}\left(|\chi(t)\rangle\otimes|\theta_0+\omega_0 t\rangle\right) = \left(i\frac{d}{dt}|\chi(t)\rangle\right))\otimes|\theta_0+\omega_0 t\rangle + |\chi(t)\rangle\otimes i\frac{d}{dt}|\theta_0+\omega_0 t\rangle \tag{124}$$

$$= \left[H(\theta_0+\omega_0 t)|\chi(t)\rangle\right]\otimes|\theta_0+\omega_0 t\rangle + |\chi(t)\rangle\otimes\left(-\omega_0\hat{l}|\theta_0+\omega_0 t\rangle\right) \tag{125}$$

$$= \left(\hat{\mathcal{H}}(\theta)-\omega_0\hat{l}\right)|\chi(t)\rangle\otimes|\theta_0+\omega_0 t\rangle. \tag{126}$$

Now, energy bands are introduced in the Floquet picture.

### C. FWS ladder for an isolated band

A single state is considered first:

$$\hat{H} = E(\hat{\theta}). \tag{127}$$

The relation $E(\theta)$ is shown schematically in Fig. 1a. Following the discussion in the preceding sections, the extended Hamiltonian takes the form

$$\tilde{H} = E(\hat{\theta}) - \omega_0\hat{l}, \tag{128}$$

which is represented schematically in Fig. 1b. The Hamiltonian given by Eq. (128) is exactly diagonalizable, whatever the "dispersion relation" $E(\theta)$.

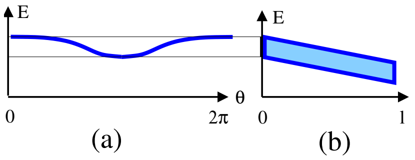


FIG. 1: *Tilted band picture for a single quantum state:* Panel a shows the schematics of $E(\theta)$ for a single quantum state [see Eq. (127]. Panel b shows how the tilted band picture in the $(l,E)$ plane is related to $E(\theta)$, with the addition of $-\omega_0 l$ in the extended Hamiltonian given by Eq. (128).

Eq. (128) is a simplified version of a two-terminal Josephson junction in which one the two Andreev bound states was removed "by hand". The auxiliary term in Eq. (128) has the meaning of adding to the superconducting Hamiltonian the term $eV(\hat{N}_a-\hat{N}_b)$, where $\hat{N}_a$ and $\hat{N}_b$ stand for the numbers of fermions in $S_a$ and $S_b$. The variable $\theta$ in Eq. (128) plays the role of the superconducting phase difference $\varphi$, and $E(\theta)$ is like the equilibrium energy-phase relation of the single Andreev bound state that was selected in this toy-model.

Coming back to Eq. (128), it is convenient to use the $\theta$-representation because $\hat{l} = i\partial/\partial\theta$. The steady states are given by

$$\left(-i\omega_0\frac{\partial}{\partial\theta}+E(\theta)\right)\psi(\theta) = E\psi(\theta). \tag{129}$$

It is deduced that energy is quantized according to $E_j = j\omega_0 + \langle E\rangle$, thus defining FWS resonance energies, which are separated by the energy quantum $\omega_0$.

Semi-classically, the eigenstates are concentrated in phase-space along curves defined by the relation $E(\theta)-\omega_0 l = E$. Wave-packets oscillate periodically with $\theta$, with an amplitude $\Delta l = \Delta E/\omega_0$, with $\Delta E$ the band-width. If $l$ is a position, or any physical degree of freedom, those oscillations are often called "Bloch oscillations". Experimentally, those have been observed in superlattices, and in cold atom systems on optical lattices.

The states are spatially extended in the limit $\omega_0 \to 0$. The spatial extent of those states can be visualized by FWS ladders of resonances for a band-structure depending on $l$ (see Fig. 2).

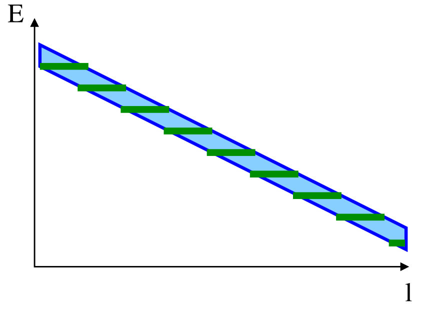


FIG. 2: *Schematics of a single FWS ladder:* The solid green lines show the energy of the FWS Andreev resonances. The length of those green lines shows the extent of the wave-functions along coordinate $l$ of the auxiliary variable.

## VII. TWO COMPLEMENTARY CALCULATIONS FOR THE RABI FREQUENCIES IN THE INFINITE-GAP LIMIT

The expression of the FWS-Andreev resonance energies is given in Eqs. (4)-(5) in the paper. Those are obtained from an especially elegant argument relying on Bohr-Sommerfeld quantization. In addition, a simple argument based on the rotating-wave approximation is also presented in connection with Eqs. (4)-(5) in the paper. Those expressions are also recovered here on the basis of Green's function calculations in a limiting case, which turn out to be much less transparent than the two other approaches. This demonstrates that Green's function calculations are not the best tool for obtaining analytical results on this problem.

### A. Schrödinger equation

The superconducting phases $\varphi_a$, $\varphi_b$ and $\varphi_c$ of leads $S_a$, $S_b$ and $S_c$ are time-independent in the equilibrium situation considered now. The two relevant Andreev bound states are then at energies $\pm\Gamma|z|$, with

$$z = \exp\left(i\varphi_a\right) + \exp\left(i\varphi_b\right) + \exp\left(i\varphi_c\right), \tag{130}$$

where it was supposed that $\Gamma/\Delta \ll 1$. The parameter $\Gamma = \Sigma^2/W$ is related to the tunnel matrix element $\Sigma$ between the dot and the superconductors, with $W$ the band-width. The wave-function for $\Gamma/\Delta \ll 1$ is described by a two-component spinor in Nambu, and its dynamics is controlled by the following $2\times 2$ Hamiltonian (see Ref. 15 for an Andreev quantum-bit):

$$\hat{\mathcal{H}}_{2\times 2}(t) = -\Gamma \left(\begin{array}{cc} 0 & z(t) \\ \overline{z}(t) & 0 \end{array}\right), \tag{131}$$

where the time-dependence of $z(t)$ in Eq. (130) was introduced for a three-terminal Josephson junction biased at $V_{a,b} = \pm V$ and $V_c = 0$.

At equilibrium, the fully dressed Green's function $\hat{G}_{x,x}$ is obtained from Dyson equation:

$$\hat{G}_{x,x} = \left(\begin{array}{cc} \omega + \Gamma\frac{\omega}{\sqrt{\Delta^2-\omega^2}} & \Gamma z \frac{\Delta}{\sqrt{\Delta^2-\omega^2}} \\ \Gamma\overline{z}\frac{\Delta}{\sqrt{\Delta^2-\omega^2}} & \omega + \Gamma\frac{\omega}{\sqrt{\Delta^2-\omega^2}} \end{array}\right)^{-1}, \tag{132}$$

where $z$ is given by Eq. (130).

In the infinite-gap limit considered in this Section, two Andreev bound states are obtained at energies $\omega_\pm = \pm\Gamma|z|$ and zero-energy states are obtained for phases $(\varphi_a^{(0)}, \varphi_b^{(0)}) = \pm(2\pi/3, -2\pi/3)$, with $\varphi_c^{(0)} = 0$ the reference phase variable, which is in agreement with Ref. 16. The fully dressed quantum dot Green's function takes the form

$$\hat{G}_{x,x} = \left(\omega - \hat{\mathcal{H}}_{2\times 2}\right)^{-1}, \tag{133}$$

with the $2\times 2$ Hamiltonian given by Eq. (131). The eigenstates are obtained by noting that the matrix residue of the Green's function corresponds to a projector on those eigenstates, which are thus given by

$$|\psi_+\rangle = \frac{1}{\sqrt{2}}\left(\begin{array}{c} \exp(i\theta) \\ -1 \end{array}\right), \text{ with } \omega_+ = \rho, \text{ and } |\psi_-\rangle = \frac{1}{\sqrt{2}}\left(\begin{array}{c} \exp(i\theta) \\ 1 \end{array}\right), \text{ with } \omega_- = -\rho, \tag{134}$$

with $z = \rho \exp(i\theta)$. The states $|\psi_\pm\rangle$ correspond to the two Andreev bound states at energies $\omega_\pm = \pm\rho$.

In the presence of applied bias voltage, the two-component wave-function is given by

$$|\psi(t)\rangle = \alpha_+(t)|\psi_+(t)\rangle + \alpha_-(t)|\psi_-(t)\rangle. \tag{135}$$

The Schrödinger equation $i|\dot{\psi}\rangle = \mathcal{H}_{2\times 2}|\psi\rangle$ becomes

$$i\begin{pmatrix} \dot{\alpha}_+ \\ \dot{\alpha}_- \end{pmatrix} = \begin{pmatrix} \omega_+ - i\langle\psi_+|\dot{\psi}_+\rangle & -i\langle\psi_+|\dot{\psi}_-\rangle \\ -i\langle\psi_-|\dot{\psi}_+\rangle & \omega_- - i\langle\psi_-|\dot{\psi}_-\rangle \end{pmatrix} \begin{pmatrix} \alpha_+ \\ \alpha_- \end{pmatrix}. \tag{136}$$

Taking into account that $\langle\psi_\sigma|\dot{\psi}_{\sigma'}\rangle = i\dot{\theta}/2$, with $\sigma, \sigma' \in \{\pm\}$ leads to

$$i\begin{pmatrix} \dot{\alpha}_+ \\ \dot{\alpha}_- \end{pmatrix} = \begin{pmatrix} \Gamma\rho + \dot{\theta}/2 & \dot{\theta}/2 \\ \dot{\theta}/2 & -\Gamma\rho + \dot{\theta}/2 \end{pmatrix} \begin{pmatrix} \alpha_+ \\ \alpha_- \end{pmatrix}. \tag{137}$$

### B. Rabi resonance from secular terms

The effective Hamiltonian in Eq. (137) is typical of atomic physics:

$$\mathcal{H}_{eff} = \mathbf{h}(t).\hat{\sigma} + \dot{\theta}\hat{I}, \tag{138}$$

where the magnetic field is given by

$$\mathbf{h}(t) = \begin{pmatrix} \dot{\theta}(t) \\ 0 \\ \Gamma\rho(t) \end{pmatrix}, \text{ and } \hat{\sigma} = \begin{pmatrix} \hat{\sigma}_x \\ \hat{\sigma}_y \\ \hat{\sigma}_z \end{pmatrix}, \tag{139}$$

where $\hat{\sigma}_{x,y,z}$ are the three Pauli matrices.

Eqs. (137) and (138) define the evolution of the wave-functions in the rotating frame. Eq. (137) implies an effective Hamiltonian $\overline{\hat{\mathcal{H}}_0} + \delta\hat{\mathcal{H}}(t)$ in the rotating frame, with

$$\overline{\hat{\mathcal{H}}_0} = \begin{pmatrix} \Gamma\overline{\rho} & 0 \\ 0 & -\Gamma\overline{\rho} \end{pmatrix} \tag{140}$$

$$\delta\hat{\mathcal{H}}(t) = \begin{pmatrix} \Gamma\delta\rho(t) + \delta\dot{\theta}(t)/2 & \delta\dot{\theta}(t)/2 \\ \delta\dot{\theta}(t)/2 & -\Gamma\delta\rho(t) + \delta\dot{\theta}(t)/2 \end{pmatrix}, \tag{141}$$

with $\rho(t) = \overline{\rho} + \delta\rho(t)$ and $\theta(t) = \overline{\theta} + \delta\theta(t)$, where the overline denotes time averaging. The Hamiltonian in the interaction representation is given by

$$\hat{\mathcal{H}}_I(t) = \exp\left(i\overline{\hat{\mathcal{H}}_0}t\right)\delta\hat{\mathcal{H}}(t)\exp\left(-i\overline{\hat{\mathcal{H}}_0}t\right). \tag{142}$$

The off-diagonal components of those $2 \times 2$ matrices are evaluated easily, with typical phase factors $\exp(2i\Gamma t)\exp(\pm i\omega_0 t)$. Imposing that those terms become static leads to a Rabi resonance at frequency $2\Gamma\overline{\rho} = \omega_0$, or, in terms of applied voltage:

$$eV_R = \Gamma\overline{\rho}, \tag{143}$$

where $V_R$ appears in Eq. (8) in the paper, and $\langle E\rangle = \Gamma\overline{\rho}$. Now Eq. (143) is demonstrated in a limiting case from Green's function calculations.

### C. Green's function calculations for $V_R$

The procedure by which the Rabi frequency can be extracted from Green's functions calculations is presented first.

The wave-functions given by Eq. (137) take the form

$$|\psi_\pm(t)\rangle = e^{\pm i\omega_{Fl}t}\sum_{m=-\infty}^{+\infty} e^{-im\omega_0 t}|\chi_{\pm,m}\rangle, \tag{144}$$

where $|\chi_{\pm,m}\rangle$ are the Floquet eigenvectors. The wave-function at time $t$ takes the form

$$|\psi(t)\rangle = \sum_{\alpha=\pm} \langle\psi_\alpha(0)|\psi(0)\rangle|\psi_\alpha(t)\rangle, \tag{145}$$

and the evolution operator is given by

$$U(t,t') = \sum_{\alpha=\pm} |\psi_\alpha(t)\rangle\langle\psi_\alpha(t')|, \tag{146}$$

from what the advanced Green's function is deduced:

$$G^A(\omega,\omega') = \sum_{\alpha=\pm}\sum_{m,n=-\infty}^{+\infty} \frac{2\pi\delta\left(\omega-\omega'-(n-m)\omega_0\right)}{\omega-\alpha\omega_{Fl}-n\omega_0-i\eta}|\chi_{\alpha,n}\rangle\langle\chi_{\alpha,m}|. \tag{147}$$

Using $n=m$ as in what follows is sufficient for obtaining the Floquet frequencies $\pm\omega_{Fl}$ as the poles of the Green's function.

Eq. (147) is valid from the quasiadiabatic to the antiadiabatic regimes. From now on, it is supposed that $S_a$ and $S_b$ are connected to the quantum dot by contacts having transparency much smaller than that with $S_c$ [this is the physical meaning of the parameter $y$ in the forthcoming Eq. (148)]. This approximation of weak ac-oscillations amounts to making a (quasiadiabatic) approximation which can be captured by Green's function perturbation theory, starting from the adiabatic basis.

### D. Random phase approximation

The numerical calculations in Ref. 17 corresponds to the approximation of a tunnel contact to the grounded superconductor, the two other contacts to voltage-biased superconductors having arbitrary transparency. The opposite limit is considered now: it is then the contacts with the two superconductors $S_{a,b}$ biased at $V_{a,b}=\pm V$ which are weakly connected to the quantum dot. This expansion in the strength of the time-dependent perturbation makes the random phase approximation (RPA) possible, in the spirit of Ref. 18 for the microscopic theory of collective modes. In this reference, an expansion is made in the small amplitude of ac-oscillations of the propagating modes in a bulk superconductor, and the poles of the Green's function define the dispersion relation of collective modes. Without generality, all information about the superconducting phase can be put in lead $S_c$: $\varphi_{a,b}(t)=\pm\omega_0 t/\hbar$, and $\varphi_c(t)=\varphi_c$. Then $z(t)$ in Eq. (130) takes the form

$$z(t) = 2y\cos(\omega_0 t) + \exp\left(i\varphi_c\right), \tag{148}$$

where $y \ll 1$ controls the strength of the time-dependent perturbation and $\omega_0 = 2eV$ is the Josephson frequency. As mentioned above, a parameter $y \ll 1$ can be obtained by assuming that the contact with $S_a$, $S_b$ have a transparency much smaller than that of the contact with $S_c$. Written in the form of Eq. (148), this set-up provides a localized coupling between the amplitude mode $2y\cos(\omega_0 t)$ and the supercurrent corresponding to $\exp(i\varphi_c)$.

The Green's function associated to the dynamics in the rotating frame is calculated now, starting from the unperturbed Green's functions $\tilde{g}_0 = \left(\omega - \overline{\hat{\mathcal{H}}_0}\right)^{-1}$, where $\overline{\hat{\mathcal{H}}_0}$ is given by Eq. (140). The term $\delta\hat{\mathcal{H}}(t)$ in Eq. (141) is treated as a perturbation corresponding to a self-energy denoted by $\tilde{\Sigma}(t)$ in what follows. In order to use a simple notation, the $\mp i0^+$ term was omitted in the advanced and retarded Green's functions respectively. The forthcoming calculation is analytical, and it is thus straightforward to restore those $\mp i0^+$ terms in all expressions.

The Dyson series takes the form

$$\tilde{G} \;=\; \tilde{g}_0 + \tilde{g}_0\tilde{\Sigma}\tilde{g}_0 + \tilde{g}_0\tilde{\Sigma}\tilde{g}_0\tilde{\Sigma}\tilde{g}_0 + \tilde{g}_0\tilde{\Sigma}\tilde{g}_0\tilde{\Sigma}\tilde{g}_0\tilde{\Sigma}\tilde{g}_0 + \tilde{g}_0\tilde{\Sigma}\tilde{g}_0\tilde{\Sigma}\tilde{g}_0\tilde{\Sigma}\tilde{g}_0\tilde{\Sigma}\tilde{g}_0 + .... \tag{149}$$

Eq. (149) is next averaged over time. The terms containing an odd number of $\tilde{\Sigma}$ are vanishingly small, and what is remaining is the following:

$$\tilde{G} \;=\; \tilde{g}_0 + +\overline{\tilde{g}_0\tilde{\Sigma}\tilde{g}_0\tilde{\Sigma}\tilde{g}_0} + \overline{\tilde{g}_0\tilde{\Sigma}\tilde{g}_0\tilde{\Sigma}} \times \overline{\tilde{g}_0\tilde{\Sigma}\tilde{g}_0\tilde{\Sigma}\tilde{g}_0} + ... = \left((\tilde{g}_0)^{-1} - \overline{\tilde{\Sigma}\tilde{g}_0\tilde{\Sigma}}\right)^{-1}, \tag{150}$$

where, in addition, time averaging was performed in a pair-wise manner (random phase approximation). The goal is now to look for resonances in $\tilde{G}$. The self-energy takes the form $\tilde{\Sigma} = \tilde{\Sigma}^+ + \tilde{\Sigma}^-$, with

$$\tilde{\Sigma}^\pm = \begin{pmatrix} \Gamma\delta\rho_\pm + \delta\dot{\theta}_\pm/2 & \delta\dot{\theta}_\pm/2 \\ \delta\dot{\theta}_\pm/2 & -\Gamma\delta\rho + \delta\dot{\theta}_\pm/2 \end{pmatrix}, \tag{151}$$

where $\tilde{\Sigma}^{\pm}$ makes a transition $n \to n \pm 1$ for the labels of harmonics of the Josephson frequency. Eq. (150) takes the form $\tilde{G} = \left(\omega - \tilde{\Sigma}_{RPA}\right)^{-1}$, with

$$\tilde{\Sigma}_{RPA} = \overline{\tilde{\mathcal{H}}_0} - \tilde{\Sigma}^{+}\tilde{g}_0\tilde{\Sigma}^{-} - \tilde{\Sigma}^{-}\tilde{g}_0\tilde{\Sigma}^{+}. \tag{152}$$

The following relation defines $\delta\rho(t)$, with $\rho(t) = \overline{\rho} + \delta\rho(t)$:

$$\rho(t) = |z(t)| = \sqrt{\left(\cos\varphi_c + 2y\cos(\omega_0 t)\right)^2 + \sin^2\varphi_c} \simeq 1 + 2y\cos\varphi_c\cos(\omega_0 t). \tag{153}$$

On the other hand,

$$\tan[\theta(t)] = \frac{\sin\varphi_c}{\cos\varphi_c + 2y\cos\omega_0 t} \tag{154}$$

leads to

$$\theta(t) \simeq \varphi_c + \delta\theta(t) \tag{155}$$
$$\delta\theta(t) \simeq -2y\sin\varphi_c\cos(\omega_0 t) \tag{156}$$
$$\delta\dot{\theta}(t) \simeq 2y\omega_0\sin\varphi_c\sin(\omega_0 t). \tag{157}$$

Then, the following is obtained:

$$\delta\rho_+(t) = \delta\rho_-(t) \simeq y\cos\varphi_c \tag{158}$$
$$\delta\dot{\theta}_+(t) = -\dot{\theta}_-(t) \simeq -iy\omega_0\sin\varphi_c, \tag{159}$$

where $\delta\rho_+$, $\delta\dot{\theta}_+$ make transitions $n \to n+1$, and $\delta\rho_-$, $\delta\dot{\theta}_-$ make transitions $n \to n-1$.

Now that the matrix elements of $\tilde{\Sigma}^{\pm}$ [see Eq. (151)] are available, the expression for the Nambu components of the RPA self-energy $\tilde{\Sigma}_{RPA}$ [see Eq. (152)] are given by:

$$\begin{aligned}\tilde{\Sigma}^{1,1}_{RPA} = {} & \Gamma\overline{\rho} - \Gamma^2\overline{\delta\rho_+\delta\rho_-}g^{+}_{1,1} - \Gamma\overline{\delta\dot{\theta}_+/2\delta\rho_-}g^{+}_{1,1} - \Gamma\overline{\delta\rho_+\delta\dot{\theta}_-/2}g^{+}_{1,1} - \overline{\delta\dot{\theta}_+/2\delta\dot{\theta}_-/2}\left[g^{+}_{1,1} + g^{+}_{2,2}\right] \\ & -\Gamma^2\overline{\delta\rho_-\delta\rho_+}g^{-}_{1,1} - \Gamma\overline{\delta\dot{\theta}_-/2\delta\rho_+}g^{-}_{1,1} - \Gamma\overline{\delta\rho_-\delta\dot{\theta}_+/2}g^{-}_{1,1} - \overline{\delta\dot{\theta}_-/2\delta\dot{\theta}_+/2}\left[g^{-}_{1,1} + g^{-}_{2,2}\right],\end{aligned} \tag{160}$$

and similar expressions hold for $\tilde{\Sigma}^{2,2}_{RPA}$, $\tilde{\Sigma}^{1,2}_{RPA}$, $\tilde{\Sigma}^{2,1}_{RPA}$.
The following notations are used:

$$g^{\pm}_{1,1} = \frac{1}{\omega - \Gamma \pm \omega_0} \tag{161}$$
$$g^{\pm}_{2,2} = \frac{1}{\omega + \Gamma \pm \omega_0}. \tag{162}$$

Using Eqs. (158) and (159) leads to the following expression for the Nambu components of $\tilde{\Sigma}_{RPA}$:

$$\tilde{\Sigma}^{1,1}_{RPA} = \Gamma - y^2\Gamma^2\cos^2\varphi_c\left(g^{+}_{1,1} + g^{-}_{1,1}\right) - \frac{1}{4}y^2\omega_0^2\sin^2\varphi_c\left(g^{+}_{1,1} + g^{-}_{1,1} + g^{+}_{2,2} + g^{-}_{2,2}\right) \tag{163}$$
$$\tilde{\Sigma}^{1,1}_{RPA} = -\Gamma - y^2\Gamma^2\cos^2\varphi_c\left(g^{+}_{2,2} + g^{-}_{2,2}\right) - \frac{1}{4}y^2\omega_0^2\sin^2\varphi_c\left(g^{+}_{1,1} + g^{-}_{1,1} + g^{+}_{2,2} + g^{-}_{2,2}\right) \tag{164}$$
$$\tilde{\Sigma}^{1,2}_{RPA} = \tilde{\Sigma}^{2,1}_{RPA} = -\frac{1}{4}y^2\omega_0^2\sin^2\varphi_c\left(g^{+}_{1,1} + g^{-}_{1,1} + g^{+}_{2,2} + g^{-}_{2,2}\right). \tag{165}$$

The resonances are obtained as a vanishing of the determinant of the Green's function. The Floquet energies take the form $\omega_{Fl} = \pm\Gamma + \delta\omega_{\pm}$, with

$$\omega_{Fl} = \pm\Gamma \mp \frac{1}{2}y^2\Gamma\frac{\omega_0^2}{4\Gamma^2 - \omega_0^2}\left[1 - \cos(\varphi_Q)\right], \tag{166}$$

having the $\varphi_Q$ periodicity characteristic of the quartet phase $\varphi_Q = \varphi_a + \varphi_b - 2\varphi_c$. Perturbation theory in the parameter $y$ breaks down if $\omega_0 = 2\Gamma$. In terms of voltage, the Rabi resonances appears at $eV_k = eV_R/k = \Gamma/k$ (with $k$ an integer), which is in agreement with Eq. (8) in the paper in the limit $y \ll 1$.

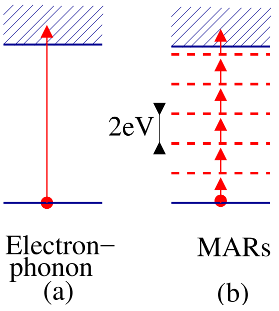


FIG. 3: *The two equilibration processes:* Panel a shows schematically a phonon process promoting an electron on the quantum dot to above the gap of one of the superconductors. Panel b shows schematically multiple Andreev reflections in analogy with multiphoton absorption. A characteristic time $\hbar/\eta_{dot}$ is associated with electron-phonon scattering on the quantum dot (panel a) and $\hbar/\eta^*_{dot}$ is the characteristic time for equilibration with the semi-infinite quasiparticle continua above the gaps by multiple Andreev reflections (panel b). (a) dominates if $\eta_{dot} \gtrsim \eta^*_{dot}$ and (b) dominates if $\eta_{dot} \lesssim \eta^*_{dot}$. It turns out that $\eta^*_{dot}$ for panel is exponentially small in $\Delta/eV$, which produces exponentially small equilibration between the quantum dot and the semi-infinite quasiparticle continua in the limit of low voltage $V$.

## VIII. CROSS-OVER BETWEEN MARS AND ELECTRON-PHONON SCATTERING

In addition to Appendix B in the paper, this section presents a physical motivation for the introduction of the nonstandard generalized Dynes parameter $\eta_{dot}$ as an imaginary part added to the energy of electrons on the quantum dot. The parameter $\eta_{dot}$ comes in addition to the standard Dynes parameter $\eta_S$ in the superconducting leads.

The Dynes parameters in the superconductors are first sources of equilibration. However, in a structure with an embedded quantum dot (see Fig. 1 in the paper), other mechanisms for equilibration are possible, with initial states on the quantum dot, not in the superconducting leads. Electron-electron interactions on the quantum dot can be neglected as a source of equilibration because of the absence of phase space for electron-electron scattering in the presence of a large energy separation between discrete levels on the quantum dot. Absorption of a phonon or MARs cooperate to couple the quantum dot degrees of freedom to the half-infinite quasiparticle continua: electron-phonon scattering takes an electron on the quantum dot and promotes it to energies larger than the gap (see Fig. 3a). MARs (see Fig. 3b) are similar to multiphoton absorption in atomic physics: the coupling to the continua is realized by a sequence of multiple Andreev reflections, each of those increasing energy by $2eV$. Electron-phonon scattering on the quantum dot is captured phenomenologically by a finite Dynes parameter $\eta_{dot}$ on the quantum dot (corresponding to a small imaginary part $\eta_{dot}$ added to the otherwise real-valued energy of electrons crossing the quantum dot). It is useful to introduce a characteristic $\eta^*_{dot}$ separating electron-phonon-dominated equilibration for $\eta_{dot} \gtrsim \eta^*_{dot}$ from MAR-dominated equilibration for $\eta_{dot} \lesssim \eta^*_{dot}$. The parameter $\eta_{dot}$ due to electron-phonon interactions is exponentially small in $\Delta/T$, the ratio between the gap $\Delta$ and temperature $T$. On the other hand, the cross-over generalized Dynes parameter $\eta^*_{dot}$ due to MARs is exponentially small in $\Delta/eV$. Two different regimes are obtained, depending on how those two parameters compare with each other, namely, on how temperature compares with voltage.

It is numerical evidence that the Dynes parameter $\eta_{dot}$ has a stronger effect on the current than the Dynes parameter $\eta_S$ [See for instance Fig. 9 in the paper, for $\eta_{dot}, \eta_S = 10^{-4}\Delta$ in comparison with $\eta_{dot}, \eta_S = 10^{-6}\Delta$]. The origin of the difference lies in the stronger efficiency of $\eta_{dot}$ than $\eta_S$ as an equilibration mechanism. For example, for a quantum dot isolated from the superconducting leads and coupled only to $\eta_{dot}$, the subgap spectral density of state at energy $\omega \gg \eta_{dot}$ is $\rho_{dot}(\omega) = \eta_{dot}/\pi\omega^2$. The latter is obtained as $\rho_{dot}(\omega) = \mathrm{Im}[g^A_{dot}(\omega)]/\pi$, where $g^A_{dot}(\omega) = 1/(\omega - i\eta_{dot})$ is the Green's function of the quantum dot. On the other hand, the normal density of states induced in the superconducting gap by electron-phonon scattering is $\rho_S = \eta_S/\pi\Delta W$, with $W$ the band-width of the superconductor. It is deduced that $\rho_{dot}(\omega) \gg \rho_S$ at subgap energies $\Delta$, because $\Delta/W \ll 1$ for superconducting materials such as Aluminum. This justifies our description based on $\eta_{dot}$: Equilibration is more efficient for processes in which a phonon is first absorbed by $\eta_{dot}$ on the quantum dot, and tunneling to the superconducting leads comes next at energies of order $\sim \Delta$. Less efficient processes are those in which an electron tunnels in the superconducting lead at low energy compared to the gap, and is next promoted to energies larger than $\sim \Delta$ by the Dynes parameter $\eta_S$. Technically, $\eta_{dot}$ and $\eta_S$ involve different numerical implementations, because $\eta_{dot}$ requires additional self-consistency loop in the presence of a finite quartet phase $\varphi_Q \neq 0$ (see Sec. III in Supplemental Material). Our calculations with finite $\eta_{dot}$ are expected to be equivalent to introducing a fourth normal lead[19]. Zero-current condition on the additional normal lead implies in this case self-consistent determination of its bias voltage, which is equivalent to the self-consistency loop implemented here. The experimental Ref. 5 involves only three superconducting leads, without fourth normal electrode, and this is why introducing $\eta_S$ and $\eta_{dot}$ appears to be more relevant than a fourth normal lead in view of discussing

all-superconducting three-terminal Josephson junctions.

A more realistic model of electron-phonon scattering would involve coupling the density of the quantum dot to a coordinate $\hat{x}$ representing lattice displacements. Then, at small $\hat{x}$, the dot energy level would oscillate without coupling to the semi-infinite quasiparticle continua, and provide a current-conserving dephasing for the electrons and holes crossing the quantum dot. This corresponds to the $\eta_{dot}$-sensitivity of the currents at $\varphi_Q = 0$, in which case current is automatically conserved with finite $\eta_{dot}$. Electrons on the quantum dot can also absorb large numbers of phonon quanta and next tunnel into the superconducting semi-infinite continua, which corresponds to processes looking like Fig. 3a, being now the result of multiphonon absorption, instead of absorption of a single phonon. This more evolved model of electron-phonon coupling may provide a different answer to the issue of current conservation, however, probably, on the basis of computationally more expansive calculations.

The exponential smallness in $\Delta/eV$ of the mechanism for equilibration with quasiparticle continua above the gaps is an incitement to demonstrate that all processes relax within a finite time window at fixed voltage (on the other extreme, spin glasses offer infinite time memory kernel). As mentioned in the paper, the coupling to the quasiparticle continua is at the origin of the exponential smallness in $\Delta/eV$ of the spectral FWS-Andreev line-width broadening. It is at this stage that introducing also the finite Dynes parameter $\eta_{dot}$ (in addition to $\eta_S$) makes the issue of equilibration rather interesting, because it relates to nonadiabaticity in the limit $eV/\Delta \to 0$. The adiabatic theorem (see Secs. I and II in Supplemental Material) corresponds to the following "abstract" statement on infinite time behavior: the currents calculated[1] with $\eta_{dot} = 0$ coincide with those evaluated for $\eta_{dot} = 0^+$. The meaning of this statement looks physically acceptable, once rephrased in a physical language: equilibration is reached after a finite (not infinite) time scale, roughly set by the minimum between $(\hbar/\eta_S,\, \hbar/\eta_{dot})$, and $(\hbar/\eta_S^*,\, \hbar/\eta_{dot}^*)$. The former are characteristic relaxation times (due to electron-electron or electron-phonon interactions), which also define the duration over which the quantum process develops. The latter is the equilibration time produced by the coupling to the semi-infinite quasiparticle continua above the gaps, due to MARs.

In a more mathematical formulation, no difficulty arises with adiabatic theorem if $\eta_{dot}/\Delta$ and $\eta_S/\Delta$ are sent to zero at fixed voltage, but taking the limits in reverse order leads to dynamics on infinite time scales, and perfect memory on initial conditions, as for the infinite gap limit. This observation is consistent the failure of the Keldysh dressing algorithm for a discrete spectrum (see Sec. IV in Supplemental Material).

---


[1] T. Jonckheere, J. Rech, T. Martin, B. Douçot, D. Feinberg, R. Mélin, *Multipair DC Josephson resonances in a biased all-superconducting bijunction*, Phys. Rev. B **87**, 214501 (2013).

[2] D. Chevallier, J. Rech, T. Jonckheere, and T. Martin, *Current and noise correlations in a double-dot Cooper-pair beam splitter*, Phys. Rev. B **83**, 125421 (2011).

[3] Y. Cohen, Y. Ronen, J.-H. Kang, M. Heiblum, D. Feinberg, R. Mélin, H. Shtrikman, *Non-local supercurrent of quartets in a three-terminal Josephson junction*, arXiv:1606.08436 (2016).

[4] C. Caroli, R. Combescot, P. Nozières, and D. Saint-James, *Direct calculation of the tunneling current*, J. Phys. C **4**, 916 (1971).

[5] C. Caroli, R. Combescot, P. Nozières, and D. Saint-James, *A direct calculation of the tunnelling current: IV. Electron-phonon interaction effects*, J. Phys. C **5**, 21 (1972).

[6] J. C. Cuevas, A. Martín-Rodero, and A. Levy Yeyati, *Hamiltonian approach to the transport properties of superconducting quantum point contacts*, Phys. Rev. B **54**, 7366 (1996).

[7] O. Parcollet and C. Hooley, *Perturbative expansion of the magnetization in the out-of-equilibrium Kondo model*, Phys. Rev. B **66**, 085315 (2002).

[8] P. Nozières, *Theory of Interacting Fermi Systems*, Benjamin New York, 1964.

[9] J.H. Shirley, *Solution of the Schrödinger equation with a Hamiltonian periodic in time*, Phys. Rev. **138**, B979 (1965).

[10] H. Sambe, *Steady states and quasienergies of a quantum-mechanical system in an oscillating field*, Phys. Rev. A **7**, 2203 (1973).

[11] M. Moskalets and M. Büttiker, *Floquet scattering theory of quantum pumps*, Phys. Rev. B **66**, 205320 (2002).

[12] L. Arrachea and M. Moskalets, *Relation between scattering-matrix and Keldysh formalisms for quantum transport driven by time-periodic fields*, Phys. Rev. B **74**, 245322 (2006).

[13] G. Stefanucci, S. Kurth, A. Rubio and E.K.U. Gross, *Time-dependent approach to electron pumping in open quantum systems*, Phys. Rev. B **77**, 075339 (2008).

[14] E.N. Bratus', V.S. Shumeiko, E.V. Bezuglyi and G. Wendin, *DC-current transport and AC Josephson effect in quantum junctions at low voltage*, Phys. Rev. B **55**, 12666 (1997).

[15] A. Zazunov, V. S. Shumeiko, E. N. Bratus, J. Lantz, and G. Wendin, *Andreev level qubit*, Phys. Rev. Lett. **90**, 087003 (2003).

[16] B. van Heck, S. Mi, and A. R. Akhmerov, *Single fermion manipulation via superconducting phase differences in multiterminal Josephson junctions*, Phys. Rev. B **90**, 155450 (2014).

[17] J. C. Cuevas and H. Pothier, *Voltage-induced Shapiro steps in a superconducting multiterminal structure*, Phys. Rev. B **75**, 174513 (2007).

[18] I.O. Kulik, O. Entin-Wohlman and R. Orbach, *Pair susceptibility and mode propagation in superconductors: A microscopic approach*, Jour. low Temp. Phys. **43**, 591 (1981).
[19] The low-voltage current in Ref. 20 was found to change strongly with a tiny coupling to a third normal lead. This numerical observation is compatible with the ultra-sensitivity of the current on a small $\eta_{dot}/\Delta$.
[20] T. Jonckheere, A. Zazunov, K. Bayandon, V. Shumeiko and T. Martin, *Non-equilibrium supercurrent through a quantum dot: current harmonics and proximity effect due to a normal metal lead*, Phys. Rev. B **80**, 184510 (2008).
